# Supplementary material for: Tensor-Train Thermo-Field Memory Kernels for Generalized Quantum Master Equations
Source: arXiv:2208.14273 source file (2022-08-31)
Supplement: Supplementary file 1 [file SI.pdf]

# Tensor-train thermo-field memory kernels for generalized quantum master equations

## Supplementary Material

Ningyi Lyu<sup>1,§</sup>, Ellen Mulvihill<sup>1,§</sup>, Micheline Soley<sup>1,2,3</sup>, Eitan Geva<sup>4,\*</sup>, and Victor Batista<sup>1,2,\*</sup>

<sup>1</sup>*Department of Chemistry, Yale University, New Haven, Connecticut 06520, United States*

<sup>2</sup>*Yale Quantum Institute, Yale University, New Haven, Connecticut 06511, United States*

<sup>3</sup>*Department of Chemistry, University of Wisconsin-Madison, Madison, Wisconsin 53706, United States*

<sup>4</sup>*Department of Chemistry, University of Michigan, Ann Arbor, Michigan 48109, United States*

<sup>§</sup>*These authors contributed equally.*

\***E-mail:** eitan@umich.edu, victor.batista@yale.edu

This supplementary material includes a thorough derivation of the GQME reduced-dimensionality approach and a description of the linear combinations used within the TT-TFD approach to obtain elements of the time evolution operator of the reduced electronic density operator,  $\mathcal{U}(t)$ , for off-diagonal initial states along with graphs of the PFIs, memory kernels, and inhomogeneous terms that are not included in the main text.

## Table of Contents

|       |                                                                                     |     |
|-------|-------------------------------------------------------------------------------------|-----|
| S.I   | GQME Derivation                                                                     | S1  |
| S.I.1 | Modified Approach to the GQME (M-GQME)                                              | S3  |
| S.I.2 | Reduced-Dimensionality GQMEs                                                        | S6  |
| S.II  | Projection-Free Inputs                                                              | S11 |
| S.III | Equivalence between the TFD Schrödinger equation and the quantum Liouville equation | S16 |
| S.IV  | Linear Combinations for Off-Diagonal Initial States of $\mathcal{U}(t)$             | S16 |
| S.V   | Graphs of the Projection-Free Inputs                                                | S18 |
| S.VI  | Graphs of the Memory Kernels                                                        | S30 |
| S.VII | Graphs of the Inhomogeneous Terms of All of the Models                              | S46 |
|       | References                                                                          | S49 |

## S.I GQME Derivation

The derivation of the GQME starts with the quantum Liouville equation (sometimes also called the von Neumann equation) for the density operator of the overall system  $\hat{\rho}(t)$ :

$$\frac{d}{dt}\hat{\rho}(t) = -\frac{i}{\hbar}\mathcal{L}\hat{\rho}(t), \quad (\text{S.1})$$

where the  $\mathcal{L} = [\hat{H}, \cdot]$  is the Liouvillian superoperator and  $\hat{H}$  is the Hamiltonian of the overall system and is assumed to be time-independent for simplicity. Throughout these notes, boldfaced variables, e.g.,  $\mathbf{A}$ , indicate vector quantities; a hat over a variable, e.g.,  $\hat{B}$ , indicates an operator quantity; and calligraphic font, e.g.,  $\mathcal{L}$ , indicates a superoperator.

The derivation of the GQME equation uses projection operator techniques. A projection operator is an operator that satisfies idempotence, i.e., additional applications of the operator do not change the result beyond the initial application of operator (e.g.,  $\hat{A}^2 = \hat{A}$ ), and is used to project on to a certain subspace of the system.

We use any projection superoperator  $\mathcal{P}$ , apply it to both sides of Eq. (S.1), and use its complimentary projection superoperator  $\mathcal{Q} = 1 - \mathcal{P}$  (i.e.,  $\mathcal{Q}$  projects onto what  $\mathcal{P}$  projects out) to reach:

$$\begin{aligned} \frac{d}{dt} \mathcal{P} \hat{\rho}(t) &= -\frac{i}{\hbar} \mathcal{P} \mathcal{L} \hat{\rho}(t) \\ &= -\frac{i}{\hbar} \mathcal{P} \mathcal{L} (\mathcal{P} + \mathcal{Q}) \hat{\rho}(t) \\ &= -\frac{i}{\hbar} \mathcal{P} \mathcal{L} \mathcal{P} \hat{\rho}(t) - \frac{i}{\hbar} \mathcal{P} \mathcal{L} \mathcal{Q} \hat{\rho}(t). \end{aligned} \quad (\text{S.2})$$

The same can be done for  $\mathcal{Q} \hat{\rho}(t)$ :

$$\frac{d}{dt} \mathcal{Q} \hat{\rho}(t) = -\frac{i}{\hbar} \mathcal{Q} \mathcal{L} \mathcal{P} \hat{\rho}(t) - \frac{i}{\hbar} \mathcal{Q} \mathcal{L} \mathcal{Q} \hat{\rho}(t), \quad (\text{S.3})$$

which, when considered as an inhomogeneous first-order differential equation, can be solved explicitly to give

$$\mathcal{Q} \hat{\rho}(t) = e^{-i\mathcal{Q}\mathcal{L}t/\hbar} \mathcal{Q} \hat{\rho}(0) - \frac{i}{\hbar} \int_0^t dt' e^{-i\mathcal{Q}\mathcal{L}(t-t')/\hbar} \mathcal{Q} \mathcal{L} \mathcal{P} \hat{\rho}(t'). \quad (\text{S.4})$$

The proof of Eq. (S.4) is done by first plugging the RHS of Eq. (S.4) into the LHS of Eq. (S.3) and evaluating the derivative, using the identity  $\frac{d}{dt} \int_0^t dt' f(t, t') = f(t, t) + \int_0^t dt' \frac{\partial f(t, t')}{\partial t}$ :

$$\begin{aligned} &\frac{d}{dt} \left\{ e^{-i\mathcal{Q}\mathcal{L}t/\hbar} \mathcal{Q} \hat{\rho}(0) - \frac{i}{\hbar} \int_0^t dt' e^{-i\mathcal{Q}\mathcal{L}(t-t')/\hbar} \mathcal{Q} \mathcal{L} \mathcal{P} \hat{\rho}(t') \right\} \\ &= -\frac{i}{\hbar} \mathcal{Q} \mathcal{L} e^{-i\mathcal{Q}\mathcal{L}t/\hbar} \mathcal{Q} \hat{\rho}(0) - \frac{i}{\hbar} \mathcal{Q} \mathcal{L} \mathcal{P} \hat{\rho}(t) - \frac{1}{\hbar^2} \int_0^t dt' \mathcal{Q} \mathcal{L} e^{-i\mathcal{Q}\mathcal{L}(t-t')/\hbar} \mathcal{Q} \mathcal{L} \mathcal{P} \hat{\rho}(t'). \end{aligned} \quad (\text{S.5})$$

We then substitute the RHS of Eq. (S.4) into the second term on the RHS of Eq. (S.3):

$$-\frac{i}{\hbar} \mathcal{Q} \mathcal{L} \mathcal{Q} \hat{\rho}(t) = -\frac{i}{\hbar} \mathcal{Q} \mathcal{L} e^{-i\mathcal{Q}\mathcal{L}t/\hbar} \mathcal{Q} \hat{\rho}(0) - \frac{1}{\hbar^2} \int_0^t dt' \mathcal{Q} \mathcal{L} e^{-i\mathcal{Q}\mathcal{L}(t-t')/\hbar} \mathcal{Q} \mathcal{L} \mathcal{P} \hat{\rho}(t'). \quad (\text{S.6})$$

If we combine the RHS of the above equation with the first, and only other, term of the RHS of Eq. (S.3),  $-\frac{i}{\hbar}\mathcal{Q}\mathcal{L}\mathcal{P}\hat{\rho}(t)$ , we can see that it is equivalent to Eq. (S.5) [which is the evaluation of the LHS of Eq. (S.3)], proving Eq. (S.4).

We then change the integration variable of Eq. (S.4) with  $t' = t - \tau$ , giving

$$\mathcal{Q}\hat{\rho}(t) = e^{-i\mathcal{Q}\mathcal{L}t/\hbar}\mathcal{Q}\hat{\rho}(0) - \frac{i}{\hbar}\int_0^t d\tau e^{-i\mathcal{Q}\mathcal{L}(\tau)/\hbar}\mathcal{Q}\mathcal{L}\mathcal{P}\hat{\rho}(t - \tau). \quad (\text{S.7})$$

Plugging Eq. (S.7) into Eq. (S.2) leads to the the Nakajima-Zwanzig equation:<sup>1-4</sup>

$$\begin{aligned} \frac{d}{dt}\mathcal{P}\hat{\rho}(t) &= -\frac{i}{\hbar}\mathcal{P}\mathcal{L}\mathcal{P}\hat{\rho}(t) - \frac{i}{\hbar}\mathcal{P}\mathcal{L}\left[e^{-i\mathcal{Q}\mathcal{L}t/\hbar}\mathcal{Q}\hat{\rho}(0) - \frac{i}{\hbar}\int_0^t d\tau e^{-i\mathcal{Q}\mathcal{L}(\tau)/\hbar}\mathcal{Q}\mathcal{L}\mathcal{P}\hat{\rho}(t - \tau)\right] \\ &= -\frac{i}{\hbar}\mathcal{P}\mathcal{L}\mathcal{P}\hat{\rho}(t) - \frac{i}{\hbar}\mathcal{P}\mathcal{L}e^{-i\mathcal{Q}\mathcal{L}t/\hbar}\mathcal{Q}\hat{\rho}(0) - \frac{1}{\hbar^2}\int_0^t d\tau \mathcal{P}\mathcal{L}e^{-i\mathcal{Q}\mathcal{L}\tau/\hbar}\mathcal{Q}\mathcal{L}\mathcal{P}\hat{\rho}(t - \tau). \end{aligned} \quad (\text{S.8})$$

Importantly, there is a lot of flexibility when it comes to the choice of projection superoperator,  $\mathcal{P}$ , and thereby observables of interest. Each such choice would in turn give rise to a different equation of motion, or GQME, for the observable quantity of interest, as dictated by the choice of projection superoperator. In Ref. 5, we explored several different projection operators that gave different GQMEs for the reduced electronic density operator and found that the modified approach to the GQME (previously introduced in Ref. 6) was the best choice. In Ref. 7, we outlined different projection operators that resulted in reduced-dimensionality GQMEs for subsets of electronic populations and/or coherences. The next two subsections will outline the modified approach to the GQME (M-GQME) and the general reduced-dimensionality GQME for any subset of the elements of the electronic reduced density matrix.

### S.I.1 Modified Approach to the GQME (M-GQME)

The modified approach to the GQME (M-GQME) gives an equation of motion for the full electronic reduced density matrix. We will assume the initial state of the overall system has the commonly-encountered factorized form

$$\hat{\rho}(0) = \hat{\rho}_n(0) \otimes \hat{\sigma}(0), \quad (\text{S.9})$$

where  $\hat{\rho}_n(0) = \text{Tr}_e\{\hat{\rho}(0)\}$  and  $\hat{\sigma}(0) = \text{Tr}_n\{\hat{\rho}(0)\}$  are the reduced density operators that describe the initial states of the nuclear DOF and electronic DOF, respectively, and  $\text{Tr}_e\{\cdot\}$  and  $\text{Tr}_n\{\cdot\}$  stand for partially tracing over the electronic Hilbert space and the nuclear Hilbert space, respectively. It should be noted that this initial state is not required for the GQME and Ref. 6 outlines a method of using the GQME approach for an entangled initial state. The M-GQME is based on the following

choice of projection superoperator:

$$\mathcal{P}^{\text{full}}(\hat{A}) = \hat{\rho}_n(0) \otimes \text{Tr}_n\{\hat{A}\} . \quad (\text{S.10})$$

Here,  $\hat{A}$  is an arbitrary overall system operator that the projection superoperator  $\mathcal{P}$  operates on and  $\hat{\rho}_n(0)$  must satisfy the condition  $\text{Tr}_n\{\hat{\rho}_n(0)\} = 1$ . If it does not, a different nuclear reference density operator can be used, as outlined in Ref. 6.

Breaking down each term in Eq. (S.8), we substitute in  $\mathcal{P}^{\text{full}} = \hat{\rho}_n(0) \otimes \text{Tr}_n\{\cdot\}$  and  $\mathcal{Q}^{\text{full}} = 1 - \mathcal{P}^{\text{full}}$  (always substituting the furthest right projection operator first, for ease of derivation) and perform a partial trace over the nuclear Hilbert space ( $\text{Tr}_n$ ) for each term:

- LHS:

$$\begin{aligned} \text{Tr}_n \left\{ \frac{d}{dt} \mathcal{P}^{\text{full}} \hat{\rho}(t) \right\} &= \frac{d}{dt} \text{Tr}_n \left\{ \hat{\rho}_n(0) \otimes \underbrace{\text{Tr}_n\{\hat{\rho}(t)\}}_{\hat{\sigma}(t)} \right\} = \frac{d}{dt} \underbrace{\text{Tr}_n \left\{ \hat{\rho}_n(0) \right\}}_1 \otimes \hat{\sigma}(t) \\ &= \boxed{\frac{d}{dt} \hat{\sigma}(t)} \end{aligned}$$

- First term RHS:

$$\text{Tr}_n \left\{ -\frac{i}{\hbar} \mathcal{P}^{\text{full}} \mathcal{L} \mathcal{P}^{\text{full}} \hat{\rho}(t) \right\} = -\frac{i}{\hbar} \text{Tr}_n \left\{ \mathcal{P}^{\text{full}} \mathcal{L} \hat{\rho}_n(0) \otimes \underbrace{\text{Tr}_n\{\hat{\rho}(t)\}}_{\hat{\sigma}(t)} \right\}$$

then we operate the first projection superoperator

$$= -\frac{i}{\hbar} \text{Tr}_n \left\{ \hat{\rho}_n(0) \otimes \text{Tr}_n \left\{ \mathcal{L} \hat{\rho}_n(0) \otimes \hat{\sigma}(t) \right\} \right\}$$

$\hat{\sigma}(t)$  is purely electronic so it can be pulled out of the  $\text{Tr}_n$  and the inner trace can be pulled out of the outer trace (since it will be purely electronic)

$$\begin{aligned} &= -\frac{i}{\hbar} \underbrace{\text{Tr}_n \left\{ \hat{\rho}_n(0) \right\}}_1 \otimes \text{Tr}_n \left\{ \mathcal{L} \hat{\rho}_n(0) \right\} \hat{\sigma}(t) \\ &= \boxed{-\frac{i}{\hbar} \langle \mathcal{L} \rangle_n^0 \hat{\sigma}(t)} \end{aligned}$$

- Second term RHS:

$$\begin{aligned}
\text{Tr}_n \left\{ \frac{i}{\hbar} \mathcal{P}^{\text{full}} \mathcal{L} e^{-i\mathcal{Q}^{\text{full}} \mathcal{L} t / \hbar} \mathcal{Q}^{\text{full}} \hat{\rho}(0) \right\} &= \text{Tr}_n \left\{ \frac{i}{\hbar} \mathcal{P}^{\text{full}} \mathcal{L} e^{-i\mathcal{Q}^{\text{full}} \mathcal{L} t / \hbar} (1 - \mathcal{P}^{\text{full}}) \hat{\rho}(0) \right\} \\
&= \text{Tr}_n \left\{ \frac{i}{\hbar} \mathcal{P}^{\text{full}} \mathcal{L} e^{-i\mathcal{Q}^{\text{full}} \mathcal{L} t / \hbar} \left( \hat{\rho}(0) - \hat{\rho}_n(0) \otimes \underbrace{\text{Tr}_n \{ \hat{\rho}(0) \}}_{\hat{\sigma}(t)} \right) \right\} \\
&= \text{Tr}_n \left\{ \frac{i}{\hbar} \mathcal{P}^{\text{full}} \mathcal{L} e^{-i\mathcal{Q}^{\text{full}} \mathcal{L} t / \hbar} \left( \underbrace{\hat{\rho}(0)}_{\hat{\rho}_n(0) \otimes \hat{\sigma}(0)} - \hat{\rho}_n(0) \otimes \hat{\sigma}(0) \right) \right\} \\
&= \boxed{0}
\end{aligned}$$

- Third term RHS:

$$\begin{aligned}
&\text{Tr}_n \left\{ \frac{1}{\hbar^2} \int_0^t d\tau \mathcal{P}^{\text{full}} \mathcal{L} e^{-i\mathcal{Q}^{\text{full}} \mathcal{L} \tau / \hbar} \mathcal{Q}^{\text{full}} \mathcal{L} \mathcal{P}^{\text{full}} \hat{\rho}(t - \tau) \right\} \\
&= \int_0^t d\tau \frac{1}{\hbar^2} \text{Tr}_n \left\{ \mathcal{P}^{\text{full}} \mathcal{L} e^{-i\mathcal{Q}^{\text{full}} \mathcal{L} \tau / \hbar} \mathcal{Q}^{\text{full}} \mathcal{L} \hat{\rho}_n(0) \otimes \underbrace{\text{Tr}_n \{ \hat{\rho}(t - \tau) \}}_{\hat{\sigma}(t - \tau)} \right\}
\end{aligned}$$

next we substitute the furthest left projection operator

$$= \int_0^t d\tau \frac{1}{\hbar^2} \text{Tr}_n \left\{ \hat{\rho}_n(0) \otimes \text{Tr}_n \left\{ \mathcal{L} e^{-i\mathcal{Q}^{\text{full}} \mathcal{L} \tau / \hbar} \mathcal{Q}^{\text{full}} \mathcal{L} \hat{\rho}_n(0) \right\} \right\} \hat{\sigma}(t - \tau)$$

taking the inner trace out of the outer trace and using  $\text{Tr}_n \{ \hat{\rho}_n(0) \} = 1$  leads to

$$= \int_0^t d\tau \frac{1}{\hbar^2} \underbrace{\text{Tr}_n \left\{ \mathcal{L} e^{-i\mathcal{Q}^{\text{full}} \mathcal{L} \tau / \hbar} \mathcal{Q}^{\text{full}} \mathcal{L} \hat{\rho}_n(0) \right\}}_{\mathcal{K}^{\text{full}}(\tau)} \hat{\sigma}(t - \tau)$$

Putting these terms back together yields the following equation of motion, or GQME, for  $\hat{\sigma}(t)$ .<sup>6</sup>

$$\frac{d}{dt} \hat{\sigma}(t) = -\frac{i}{\hbar} \langle \mathcal{L} \rangle_n^0 \hat{\sigma}(t) - \int_0^t d\tau \mathcal{K}^{\text{full}}(\tau) \hat{\sigma}(t - \tau). \quad (\text{S.11})$$

Within this GQME, the effect of the projected-out nuclear DOF on the dynamics of  $\hat{\sigma}(t)$  is fully accounted for by two electronic superoperators:

- *The projected Liouvillian,*

$$\langle \mathcal{L} \rangle_n^0 \equiv \text{Tr}_n \{ \hat{\rho}_n(0) \mathcal{L} \} \quad (\text{S.12})$$

which can be represented by a *time-independent*  $N_e^2 \times N_e^2$  matrix, and

- *The memory kernel,*

$$\mathcal{K}^{\text{full}}(\tau) = \frac{1}{\hbar^2} \text{Tr}_n \left\{ \mathcal{L} e^{-i\mathcal{Q}^{\text{full}}\mathcal{L}\tau/\hbar} \mathcal{Q}^{\text{full}} \mathcal{L} \hat{\rho}_n(0) \right\}, \quad (\text{S.13})$$

which can be represented by a *time-dependent*  $N_e^2 \times N_e^2$  matrix.

While calculating the matrix elements of  $\langle \mathcal{L} \rangle_n^0$  is straightforward, this is not the case for the matrix elements of  $\mathcal{K}^{\text{full}}(\tau)$ . The memory kernel of the GQME cannot be obtained directly due to its projected dynamics, seen in the presence of the projection operator  $\mathcal{Q}$  in its exponential,  $e^{-i\mathcal{Q}\mathcal{L}\tau/\hbar}$  [see Eq. (S.13)]. Significant effort over the last two decades has been directed at developing, testing, and applying various computational schemes for calculating  $\mathcal{K}^{\text{full}}(\tau)$ . Those schemes were all based on the fact that  $\mathcal{K}^{\text{full}}(\tau)$  can be obtained from projection-free inputs (PFIs) by solving integral Volterra equations, as was first shown in Refs. 8–11. The PFIs can be calculated using either quantum-mechanically exact or approximate semiclassical and mixed quantum-classical input methods.<sup>8–23,6,24,25,5</sup> Additional studies advanced the understanding of the pros and cons of different implementations and expanded the range of applications of such GQMEs.<sup>12–23,6,24,25,5</sup> Further details on obtaining the M-GQME memory kernel from projection-free inputs will be outlined in Sec. S.II.

## S.I.2 Reduced-Dimensionality GQMEs

In this section, we explore an alternative approach for scaling up the GQME approach which is based on utilizing the flexibility offered by the GQME formalism with respect to the choice of projection operator. To this end, we use the fact that it is possible to derive a GQME for *any* subset of electronic reduced density matrix elements of one's choice. It should be noted that a similar approach has been previously discussed in Refs. 26 and 19.

In this subsection, we consider the case where the electronic observables of interest correspond to a subset of the electronic reduced density matrix elements,  $\{\sigma_{ab}(t)\}$ . The equation of motion for  $\{\sigma_{ab}(t)\}$  is obtained by using the following projection superoperator:

$$\mathcal{P}^{\text{set}} \hat{A} = \sum_{jk \in \{ab\}} \mathcal{P}^{jk} \hat{A} = \sum_{jk \in \{ab\}} \hat{\rho}_n(0) \otimes |j\rangle \langle k| \text{Tr} \left\{ \left( |k\rangle \langle j| \otimes \hat{1}_n \right) \hat{A} \right\}. \quad (\text{S.14})$$

For ease of the derivation later, we note that this projection operator when applied to the overall

system density operator gives

$$\begin{aligned}
\mathcal{P}^{\text{set}} \hat{\rho}(t) &= \sum_{jk \in \{ab\}} \hat{\rho}_n(0) \otimes |j\rangle\langle k| \text{Tr} \left\{ \left( |k\rangle\langle j| \otimes \hat{1}_n \right) \hat{\rho}(t) \right\} \\
&= \sum_{jk \in \{ab\}} \hat{\rho}_n(0) \otimes |j\rangle\langle k| \text{Tr}_e \left\{ \langle j| \text{Tr}_n \left\{ \hat{1}_n \hat{\rho}(t) \right\} |k\rangle \right\} \\
&= \sum_{jk \in \{ab\}} \hat{\rho}_n(0) \otimes |j\rangle\langle k| \text{Tr}_e \left\{ \langle j| \hat{\sigma}(t) |k\rangle \right\} \\
&= \hat{\rho}_n(0) \otimes |j\rangle\langle k| \sigma_{jk}(t)
\end{aligned} \tag{S.15}$$

For the derivation of the subset GQME, we first write Eq. (S.8) with  $\mathcal{P}^{\text{set}}$  and split into terms:

$$\begin{aligned}
\underbrace{\frac{d}{dt} \mathcal{P}^{\text{set}} \hat{\rho}(t)}_{(1)} &= \underbrace{-\frac{i}{\hbar} \mathcal{P}^{\text{set}} \mathcal{L} \mathcal{P}^{\text{set}} \hat{\rho}(t)}_{(2)} - \underbrace{\frac{1}{\hbar^2} \int_0^t d\tau \mathcal{P}^{\text{set}} \mathcal{L} e^{-i\mathcal{Q}^{\text{set}} \mathcal{L} \tau / \hbar} \mathcal{Q}^{\text{set}} \mathcal{L} \mathcal{P}^{\text{set}} \hat{\rho}(t - \tau)}_{(3)} \\
&\quad - \underbrace{\frac{i}{\hbar} \mathcal{P}^{\text{set}} \mathcal{L} e^{-i\mathcal{Q}^{\text{set}} \mathcal{L} t / \hbar} \mathcal{Q}^{\text{set}} \hat{\rho}(0)}_{(4)},
\end{aligned} \tag{S.16}$$

where  $\mathcal{Q}^{\text{set}} = 1 - \mathcal{P}^{\text{set}}$  is the complimentary projection operator to  $\mathcal{P}^{\text{set}}$  (i.e.,  $\mathcal{Q}^{\text{set}}$  projects-in what  $\mathcal{P}^{\text{set}}$  projects-out).

Plugging in the projection operator from Eq. (S.14) [always starting with the furthest right projection operator and using Eq. (S.15):  $\mathcal{P}^{\text{set}} \hat{\rho}(t) = \hat{\rho}_n(0) \otimes |j\rangle\langle k| \sigma_{jk}(t)$ ] and tracing over the nuclear DOF, we get the following for each term:

$$\begin{aligned}
(1) \quad \text{Tr}_n \left\{ \frac{d}{dt} \mathcal{P}^{\text{set}} \hat{\rho}(t) \right\} &= \frac{d}{dt} \text{Tr}_n \left\{ \sum_{jk \in \{ab\}} \hat{\rho}_n(0) \otimes |j\rangle\langle k| \sigma_{jk}(t) \right\} \\
&= \frac{d}{dt} \sum_{jk \in \{ab\}} \text{Tr}_n \left\{ \hat{\rho}_n(0) \right\} |j\rangle\langle k| \sigma_{jk}(t) \\
&= \boxed{\sum_{jk \in \{ab\}} |j\rangle\langle k| \frac{d}{dt} \sigma_{jk}(t)}
\end{aligned} \tag{S.17}$$

(2)

$$\begin{aligned}
\text{Tr}_n \left\{ -\frac{i}{\hbar} \mathcal{P}^{\text{set}} \mathcal{L} \mathcal{P}^{\text{set}} \hat{\rho}(t) \right\} &= -\frac{i}{\hbar} \text{Tr}_n \left\{ \mathcal{P}^{\text{set}} \mathcal{L} \sum_{lm \in \{ab\}} \hat{\rho}_n(0) \otimes |l\rangle \langle m| \sigma_{lm}(t) \right\} \\
&= -\frac{i}{\hbar} \sum_{\substack{jk \in \{ab\} \\ lm \in \{ab\}}} \text{Tr}_n \left\{ |j\rangle \langle k| \otimes \hat{\rho}_n(0) \underbrace{\text{Tr} \left\{ \left( |k\rangle \langle j| \otimes \hat{1}_n \right) \mathcal{L} \hat{\rho}_n(0) |l\rangle \langle m| \right\}}_{\left\langle \mathcal{L}_{jk,lm} \right\rangle_n^0} \sigma_{lm}(t) \right\}
\end{aligned}$$

the  $\text{Tr}_n$  can pass over  $|j\rangle \langle k|$  because it is purely electronic and it can pass over  $\langle \mathcal{L}_{jk,lm} \rangle_n^0$  and  $\sigma_{lm}(t)$  because they are numbers

$$\begin{aligned}
&= -\frac{i}{\hbar} \sum_{\substack{jk \in \{ab\} \\ lm \in \{ab\}}} |j\rangle \langle k| \underbrace{\text{Tr}_n \left\{ \hat{\rho}_n(0) \right\}}_1 \left\langle \mathcal{L}_{jk,lm} \right\rangle_n^0 \sigma_{lm}(t) \\
&= \boxed{-\frac{i}{\hbar} \sum_{\substack{jk \in \{ab\} \\ lm \in \{ab\}}} |j\rangle \langle k| \left\langle \mathcal{L}_{jk,lm} \right\rangle_n^0 \sigma_{lm}(t)} \tag{S.18}
\end{aligned}$$

(3)

$$\begin{aligned} \text{Tr}_n \left\{ -\frac{1}{\hbar^2} \int_0^t d\tau \mathcal{P}^{\text{set}} \mathcal{L} e^{-i\mathcal{Q}^{\text{set}} \mathcal{L} \tau / \hbar} \mathcal{Q}^{\text{set}} \mathcal{L} \mathcal{P}^{\text{set}} \hat{\rho}(t - \tau) \right\} \\ = - \int_0^t d\tau \frac{1}{\hbar^2} \text{Tr}_n \left\{ \mathcal{P}^{\text{set}} \mathcal{L} e^{-i\mathcal{Q}^{\text{set}} \mathcal{L} \tau / \hbar} \mathcal{Q}^{\text{set}} \mathcal{L} \sum_{lm \in \{ab\}} \hat{\rho}_n(0) \otimes |l\rangle \langle m| \sigma_{lm}(t - \tau) \right\} \end{aligned}$$

next, plugging in the furthest left projection operator

$$\begin{aligned} = - \int_0^t d\tau \sum_{\substack{jk \in \{ab\} \\ lm \in \{ab\}}} \frac{1}{\hbar^2} \text{Tr}_n \left\{ |j\rangle \langle k| \otimes \hat{\rho}_n(0) \right. \\ \left. \times \text{Tr} \left\{ \left( |k\rangle \langle j| \otimes \hat{1}_n \right) \mathcal{L} e^{-i\mathcal{Q}^{\text{set}} \mathcal{L} \tau / \hbar} \mathcal{Q}^{\text{set}} \mathcal{L} \hat{\rho}_n(0) \otimes |l\rangle \langle m| \sigma_{lm}(t - \tau) \right\} \right\} \end{aligned}$$

the  $\text{Tr}_n$  can pass over  $|j\rangle \langle k|$  because it is purely electronic and

it can pass over the full trace because it is a number

$$\begin{aligned} = - \int_0^t d\tau \sum_{\substack{jk \in \{ab\} \\ lm \in \{ab\}}} |j\rangle \langle k| \underbrace{\text{Tr}_n \left\{ \hat{\rho}_n(0) \right\}}_1 \\ \times \frac{1}{\hbar^2} \text{Tr} \left\{ \left( |k\rangle \langle j| \otimes \hat{1}_n \right) \mathcal{L} e^{-i\mathcal{Q}^{\text{set}} \mathcal{L} \tau / \hbar} \mathcal{Q}^{\text{set}} \mathcal{L} \hat{\rho}_n(0) \otimes |l\rangle \langle m| \sigma_{lm}(t - \tau) \right\} \end{aligned}$$

the  $\sigma_{lm}(t - \tau)$  can be taken out of the full trace because it is a number

$$= - \sum_{\substack{jk \in \{ab\} \\ lm \in \{ab\}}} |j\rangle \langle k| \int_0^t d\tau \frac{1}{\hbar^2} \text{Tr} \left\{ \underbrace{\left( |k\rangle \langle j| \otimes \hat{1}_n \right) \mathcal{L} e^{-i\mathcal{Q}^{\text{set}} \mathcal{L} \tau / \hbar} \mathcal{Q}^{\text{set}} \mathcal{L} \left( \hat{\rho}_n(0) \otimes |l\rangle \langle m| \right)}_{\mathcal{K}_{jk,lm}^{\text{set}}(\tau)} \right\} \sigma_{lm}(t - \tau)$$

(S.19)

(4)

$$\begin{aligned}
\text{Tr}_n \left\{ -\frac{i}{\hbar} \mathcal{P}^{\text{set}} \mathcal{L} e^{-i\mathcal{Q}^{\text{set}} \mathcal{L} t / \hbar} \mathcal{Q}^{\text{set}} \hat{\rho}(0) \right\} &= -\frac{i}{\hbar} \text{Tr}_n \left\{ \mathcal{P}^{\text{set}} \mathcal{L} e^{-i\mathcal{Q}^{\text{set}} \mathcal{L} t / \hbar} \left( 1 - \mathcal{P}^{\text{set}} \right) \hat{\rho}(0) \right\} \\
&\quad \text{distributing } (1 - \mathcal{P}^{\text{set}}) \hat{\rho}(0) \\
&= -\frac{i}{\hbar} \text{Tr}_n \left\{ \mathcal{P}^{\text{set}} \mathcal{L} e^{-i\mathcal{Q}^{\text{set}} \mathcal{L} t / \hbar} \left[ \hat{\rho}(0) - \sum_{lm \in \{ab\}} \hat{\rho}_n(0) \otimes |l\rangle\langle m| \sigma_{lm}(0) \right] \right\} \\
&\quad \text{plugging in the furthest left projection operator} \\
&= -\frac{i}{\hbar} \sum_{jk \in \{ab\}} \text{Tr}_n \left\{ |j\rangle\langle k| \otimes \hat{\rho}_n(0) \text{Tr} \left\{ \left( |k\rangle\langle j| \otimes \hat{1}_n \right) \mathcal{L} e^{-i\mathcal{Q}^{\text{set}} \mathcal{L} t / \hbar} \left[ \hat{\rho}(0) - \sum_{lm \in \{ab\}} \hat{\rho}_n(0) \otimes |l\rangle\langle m| \sigma_{lm}(0) \right] \right\} \right\} \\
&\quad \text{the } \text{Tr}_n \text{ can pass over } |j\rangle\langle k| \text{ because it is purely electronic and} \\
&\quad \text{it can pass over the full trace because it is a number} \\
&= -\frac{i}{\hbar} \sum_{jk \in \{ab\}} |j\rangle\langle k| \underbrace{\text{Tr}_n \left\{ \hat{\rho}_n(0) \right\}}_1 \text{Tr} \left\{ \left( |k\rangle\langle j| \otimes \hat{1}_n \right) \mathcal{L} e^{-i\mathcal{Q}^{\text{set}} \mathcal{L} t / \hbar} \left[ \hat{\rho}(0) - \sum_{lm \in \{ab\}} \hat{\rho}_n(0) \otimes |l\rangle\langle m| \sigma_{lm}(0) \right] \right\} \\
&= \sum_{jk \in \{ab\}} |j\rangle\langle k| \underbrace{\left[ -\frac{i}{\hbar} \text{Tr} \left\{ \left( |k\rangle\langle j| \otimes \hat{1}_n \right) \mathcal{L} e^{-i\mathcal{Q}^{\text{set}} \mathcal{L} t / \hbar} \left[ \hat{\rho}(0) - \sum_{lm \in \{ab\}} \hat{\rho}_n(0) \otimes |l\rangle\langle m| \sigma_{lm}(0) \right] \right\} \right]}_{I_{jk}^{\text{set}}(t)} \\
&\hspace{25em} \text{(S.20)}
\end{aligned}$$

So this term goes to zero if  $\hat{\rho}_n(0) = \sum_{lm \in \{ab\}} \hat{\rho}_n(0) \otimes \sigma_{lm}(0) |l\rangle\langle m|$ . This can often easily be true if the system starts in one population, with the rest equal to zero, and this population is included in the subset of states of interest. In other words, if  $\hat{\rho}(0) = \hat{\rho}_n(0) \otimes |\alpha\rangle\langle\alpha|$  and  $\alpha \in \{ab\}$ , then  $I_{jk}^{\text{set}}(t) = 0$ .

Therefore, the overall GQME is given by

$$\begin{aligned}
\sum_{jk \in \{ab\}} |j\rangle\langle k| \frac{d}{dt} \sigma_{jk}(t) &= -\frac{i}{\hbar} \sum_{\substack{jk \in \{ab\} \\ lm \in \{ab\}}} |j\rangle\langle k| \langle \mathcal{L}_{jk,lm} \rangle_n^0 \sigma_{lm}(t) \\
&\quad - \sum_{\substack{jk \in \{ab\} \\ lm \in \{ab\}}} |j\rangle\langle k| \int_0^t d\tau \mathcal{K}_{jk,lm}^{\text{set}}(\tau) \sigma_{lm}(t - \tau) + \sum_{jk \in \{ab\}} |j\rangle\langle k| \hat{I}_{jk}^{\text{set}}(t),
\end{aligned} \tag{S.21}$$

where the memory kernel matrix elements are given by

$$\mathcal{K}_{jk,lm}^{\text{set}}(\tau) = \frac{1}{\hbar^2} \text{Tr} \left\{ \left( |k\rangle\langle j| \otimes \hat{1}_n \right) \mathcal{L} e^{-i\mathcal{Q}^{\text{set}} \mathcal{L} \tau / \hbar} \mathcal{Q}^{\text{set}} \mathcal{L} \hat{\rho}_n(0) \otimes |l\rangle\langle m| \right\} \quad (\text{S.22})$$

and the inhomogeneous term vector elements are given by

$$\hat{I}_{jk}^{\text{set}}(t) = -\frac{i}{\hbar} \text{Tr} \left\{ \left( |k\rangle\langle j| \otimes \hat{1}_n \right) \mathcal{L} e^{-i\mathcal{Q}^{\text{set}} \mathcal{L} t / \hbar} \left[ \hat{\rho}(0) - \sum_{lm \in \{ab\}} \hat{\rho}_n(0) \otimes |l\rangle\langle m| \sigma_{lm}(0) \right] \right\}. \quad (\text{S.23})$$

Given  $N_{\text{set}}$  equal to the number of elements in  $\{\sigma_{ab}(t)\}$ , the memory kernel and inhomogeneous term in this case correspond to an  $N_{\text{set}} \times N_{\text{set}}$  matrix and an  $N_{\text{set}}$ -dimensional vector, respectively. If the initial state is of the commonly encountered factored form  $\hat{\rho}(0) = \hat{\rho}_n(0) \otimes |\alpha\rangle\langle\beta|$  and  $\alpha\beta \in \{ab\}$ , then  $\hat{I}^{\text{set}}(t) = 0$ .

## S.II Projection-Free Inputs

The memory kernels and inhomogeneous terms of the M-GQME and reduced-dimensionality GQMEs can be found via integral Volterra equations with PFIs.

For the M-GQME, a scheme for evaluating  $\mathcal{K}^{\text{full}}(\tau)$  from projection-free inputs can be developed by using the following general operator identity:<sup>8,10</sup>

$$e^{-i\mathcal{B}\tau/\hbar} = e^{-i\mathcal{A}\tau/\hbar} - \frac{i}{\hbar} \int_0^\tau d\tau' e^{-i\mathcal{A}(\tau-\tau')/\hbar} (\mathcal{B} - \mathcal{A}) e^{-i\mathcal{B}\tau'/\hbar}. \quad (\text{S.24})$$

The proof of this identity can be shown by first starting with the differential equation

$$\begin{aligned} \frac{d}{d\tau} e^{i\mathcal{A}\tau/\hbar} e^{-i\mathcal{B}\tau/\hbar} &= \left( \frac{i}{\hbar} \mathcal{A} e^{i\mathcal{A}\tau/\hbar} \right) e^{-i\mathcal{B}\tau/\hbar} + e^{i\mathcal{A}\tau/\hbar} \left( -\frac{i}{\hbar} \mathcal{B} e^{-i\mathcal{B}\tau/\hbar} \right) \quad \text{product rule} \\ &= \frac{i}{\hbar} e^{i\mathcal{A}\tau/\hbar} (\mathcal{A} - \mathcal{B}) e^{-i\mathcal{B}\tau/\hbar}. \quad \mathcal{A} \text{ and } e^{i\mathcal{A}\tau/\hbar} \text{ commute, then gathering terms} \end{aligned}$$

Integrating both sides from 0 to  $t$  leads to

$$\int_0^t d\tau \frac{d}{d\tau} e^{i\mathcal{A}\tau/\hbar} e^{-i\mathcal{B}\tau/\hbar} = \int_0^t d\tau \frac{i}{\hbar} e^{i\mathcal{A}\tau/\hbar} (\mathcal{A} - \mathcal{B}) e^{-i\mathcal{B}\tau/\hbar}$$

evaluating the LHS and flipping the sign of the integral on the RHS

$$e^{i\mathcal{A}t/\hbar} e^{-i\mathcal{B}t/\hbar} - 1 = -\frac{i}{\hbar} \int_0^t d\tau e^{i\mathcal{A}\tau/\hbar} (\mathcal{B} - \mathcal{A}) e^{-i\mathcal{B}\tau/\hbar}$$

multiplying from the left with  $e^{-i\mathcal{A}t/\hbar}$  and moving the second term on the LHS to the RHS

$$e^{-i\mathcal{B}t/\hbar} = e^{-i\mathcal{A}t/\hbar} - \frac{i}{\hbar} \int_0^t d\tau e^{-i\mathcal{A}(t-\tau)/\hbar} (\mathcal{B} - \mathcal{A}) e^{-i\mathcal{B}\tau/\hbar} \quad (\text{S.25})$$

This is equivalent to Eq. (S.24), proving the general operator identity.

Substituting  $\mathcal{A} = \mathcal{L}$  and  $\mathcal{B} = \mathcal{Q}\mathcal{L}$  into Eq. (S.24), we obtain

$$e^{-i\mathcal{Q}\mathcal{L}\tau/\hbar} = e^{-i\mathcal{L}\tau/\hbar} + \frac{i}{\hbar} \int_0^\tau d\tau' e^{-i\mathcal{L}(\tau-\tau')/\hbar} \mathcal{P} \mathcal{L} e^{-i\mathcal{Q}\mathcal{L}\tau'/\hbar}. \quad (\text{S.26})$$

Substituting Eq. (S.26) into Eq. (S.13) gives

$$\begin{aligned} \mathcal{K}^{\text{full}}(\tau) &= \frac{1}{\hbar^2} \text{Tr}_n \left\{ \mathcal{L} e^{-i\mathcal{Q}^{\text{full}}\mathcal{L}\tau/\hbar} \mathcal{Q}^{\text{full}} \mathcal{L} \hat{\rho}_n(0) \right\} \\ &= \frac{1}{\hbar^2} \text{Tr}_n \left\{ \mathcal{L} e^{-i\mathcal{L}\tau/\hbar} \mathcal{Q}^{\text{full}} \mathcal{L} \hat{\rho}_n(0) \right\} \\ &\quad + \frac{i}{\hbar^3} \int_0^\tau d\tau' \text{Tr}_n \left\{ \mathcal{L} e^{-i\mathcal{L}(\tau-\tau')/\hbar} \mathcal{P}^{\text{full}} \mathcal{L} e^{-i\mathcal{Q}^{\text{full}}\mathcal{L}\tau'/\hbar} \mathcal{Q}^{\text{full}} \mathcal{L} \hat{\rho}_n(0) \right\} \end{aligned}$$

plugging in  $\mathcal{Q}^{\text{full}} = 1 - \mathcal{P}^{\text{full}}$  in the first term and  $\mathcal{P}^{\text{full}}$  into the second term

$$\begin{aligned} &= \frac{1}{\hbar^2} \text{Tr}_n \left\{ \mathcal{L} e^{-i\mathcal{L}\tau/\hbar} (1 - \mathcal{P}^{\text{full}}) \mathcal{L} \hat{\rho}_n(0) \right\} \\ &\quad + \frac{i}{\hbar^3} \int_0^\tau d\tau' \text{Tr}_n \left\{ \mathcal{L} e^{-i\mathcal{L}(\tau-\tau')/\hbar} \hat{\rho}_n(0) \otimes \text{Tr}_n \left\{ \mathcal{L} e^{-i\mathcal{Q}^{\text{full}}\mathcal{L}\tau'/\hbar} \mathcal{Q}^{\text{full}} \mathcal{L} \hat{\rho}_n(0) \right\} \right\} \end{aligned}$$

distributing over the parentheses, plugging in  $\mathcal{P}^{\text{full}}$  in the new second term and splitting the nuclear traces in the integral term

$$\begin{aligned} &= \underbrace{\frac{1}{\hbar^2} \text{Tr}_n \left\{ \mathcal{L} e^{-i\mathcal{L}\tau/\hbar} \mathcal{L} \hat{\rho}_n(0) \right\}}_{i\dot{\mathcal{F}}(\tau)} - \underbrace{\frac{1}{\hbar} \frac{1}{\hbar} \text{Tr}_n \left\{ \mathcal{L} e^{-i\mathcal{L}\tau/\hbar} \hat{\rho}_n(0) \right\}}_{\mathcal{F}(\tau)} \underbrace{\text{Tr}_n \left\{ \mathcal{L} \hat{\rho}_n(0) \right\}}_{\langle \mathcal{L} \rangle_n^0} \\ &\quad + i \int_0^\tau d\tau' \underbrace{\frac{1}{\hbar} \text{Tr}_n \left\{ \mathcal{L} e^{-i\mathcal{L}(\tau-\tau')/\hbar} \hat{\rho}_n(0) \right\}}_{\mathcal{F}(\tau-\tau')} \underbrace{\frac{1}{\hbar^2} \text{Tr}_n \left\{ \mathcal{L} e^{-i\mathcal{Q}^{\text{full}}\mathcal{L}\tau'/\hbar} \mathcal{Q}^{\text{full}} \mathcal{L} \hat{\rho}_n(0) \right\}}_{\mathcal{K}^{\text{full}}(\tau')} \end{aligned}$$

Therefore, the full memory kernel can be found by solving the following Volterra equation of the second kind:

$$\mathcal{K}^{\text{full}}(\tau) = i\dot{\mathcal{F}}(\tau) - \frac{1}{\hbar}\mathcal{F}(\tau)\langle\mathcal{L}\rangle_n^0 + i\int_0^\tau d\tau'\mathcal{F}(\tau-\tau')\mathcal{K}^{\text{full}}(\tau'), \quad (\text{S.27})$$

where  $\mathcal{F}(\tau)$  and  $\dot{\mathcal{F}}(\tau)$  are the PFIs given by

$$\begin{aligned} \mathcal{F}(\tau) &= \frac{1}{\hbar}\text{Tr}_n\left\{\mathcal{L}e^{-i\mathcal{L}\tau/\hbar}\hat{\rho}_n(0)\right\}, \\ \dot{\mathcal{F}}(\tau) &= -\frac{i}{\hbar^2}\text{Tr}_n\left\{\mathcal{L}e^{-i\mathcal{L}\tau/\hbar}\mathcal{L}\hat{\rho}_n(0)\right\}. \end{aligned} \quad (\text{S.28})$$

Thus, given the PFIs, Eq. (S.27) can be solved numerically for the projection-dependent  $\mathcal{K}(\tau)$  (see Appendix D of Ref. 6). Hence, the problem of calculating  $\mathcal{K}(\tau)$  translates into that of calculating  $\mathcal{F}(\tau)$  and  $\dot{\mathcal{F}}(\tau)$ .

It should be noted that  $\mathcal{F}(\tau) = i\dot{\mathcal{U}}(\tau)$ , where  $\mathcal{U}(\tau)$  is the time evolution operator of the electronic reduced density operator,

$$\hat{\sigma}(\tau) = \mathcal{U}(\tau)\hat{\sigma}(0) \equiv \text{Tr}_n\left\{e^{-i\mathcal{L}\tau/\hbar}\hat{\rho}_n(0)\right\}\hat{\sigma}(0). \quad (\text{S.29})$$

Thus, Eq. (S.27) can be rewritten in the following form:

$$\mathcal{K}^{\text{full}}(\tau) = -\ddot{\mathcal{U}}(\tau) - \frac{i}{\hbar}\dot{\mathcal{U}}(\tau)\langle\mathcal{L}\rangle_n^0 - \int_0^\tau d\tau'\dot{\mathcal{U}}(\tau-\tau')\mathcal{K}^{\text{full}}(\tau'). \quad (\text{S.30})$$

This implies that the memory kernel of the M-GQME,  $\mathcal{K}^{\text{full}}(\tau)$ , can be obtained directly from the time evolution operator of the reduced dynamics,  $\mathcal{U}(\tau)$ . As shown in Ref. 5, when approximate input methods are used, the PFIs  $\mathcal{F}(\tau)$  and  $\dot{\mathcal{F}}(\tau)$  should be calculated explicitly in order to achieve the accuracy benefit of the GQME. However, with an exact input method, the time evolution operator of the reduced dynamics,  $\mathcal{U}(\tau)$ , can be used along with a numerical derivative method.

For the reduced-dimensionality GQMEs, the memory kernel  $\{\mathcal{K}^{\text{set}}(\tau)\}$  can also be obtained from PFIs by solving a set of  $N_{\text{set}}^2$  coupled Volterra equations. We start with the explicit expression for the memory kernel, Eq. (S.22):

$\mathcal{K}_{jk,lm}^{\text{set}}(\tau) = \frac{1}{\hbar^2}\text{Tr}\left\{\left(|k\rangle\langle j|\otimes\hat{1}_n\right)\mathcal{L}e^{-i\mathcal{Q}^{\text{set}}\mathcal{L}\tau/\hbar}\mathcal{Q}^{\text{set}}\mathcal{L}\hat{\rho}_n(0)\otimes|l\rangle\langle m|\right\}$ . We then substitute the identity in Eq. (S.26) for  $e^{-i\mathcal{Q}^{\text{set}}\mathcal{L}\tau/\hbar}$  (the identity is valid for any projection superoperator  $\mathcal{Q}$ ). This yields

the following expression for the matrix elements of  $\mathcal{K}^{\text{set}}(\tau)$ :

$$\begin{aligned}\mathcal{K}_{jk,lm}^{\text{set}}(\tau) = & \frac{1}{\hbar^2} \text{Tr} \left\{ \left( |k\rangle\langle j| \otimes \hat{1}_n \right) \mathcal{L} e^{-i\mathcal{L}\tau/\hbar} \mathcal{Q}^{\text{set}} \mathcal{L} \hat{\rho}_n(0) \otimes |l\rangle\langle m| \right\} \\ & + \frac{i}{\hbar^3} \int_0^\tau d\tau' \text{Tr} \left\{ \left( |k\rangle\langle j| \otimes \hat{1}_n \right) \mathcal{L} e^{-i\mathcal{L}(\tau-\tau')/\hbar} \mathcal{P}^{\text{set}} \mathcal{L} e^{-i\mathcal{Q}^{\text{set}}\mathcal{L}\tau'/\hbar} \mathcal{Q}^{\text{set}} \mathcal{L} \hat{\rho}_n(0) \otimes |l\rangle\langle m| \right\}.\end{aligned}$$

Plugging in  $\mathcal{Q}^{\text{set}} = 1 - \mathcal{P}^{\text{set}}$  into the first term splits it into two terms. Using  $\mathcal{P}^{\text{set}}$  from Eq. (S.14) in the term that involves  $\mathcal{P}^{\text{set}}$  leads to Eq. (S.31):

$$\begin{aligned}\mathcal{K}_{jk,lm}^{\text{set}}(\tau) = & \underbrace{\frac{1}{\hbar^2} \text{Tr} \left\{ \left( |k\rangle\langle j| \otimes \hat{1}_n \right) \mathcal{L} e^{-i\mathcal{L}\tau/\hbar} \mathcal{L} \hat{\rho}_n(0) \otimes |l\rangle\langle m| \right\}}_{i\dot{\mathcal{F}}_{jk,lm}(\tau)} \\ & - \frac{1}{\hbar} \sum_{uv \in \{ab\}} \underbrace{\frac{1}{\hbar} \text{Tr} \left\{ \left( |j\rangle\langle j| \otimes \hat{1}_n \right) \mathcal{L} e^{-i\mathcal{L}\tau/\hbar} \hat{\rho}_n(0) \otimes |u\rangle\langle v| \right\}}_{\mathcal{F}_{jk,uv}(\tau)} \underbrace{\text{Tr} \left\{ \left( |v\rangle\langle u| \otimes \hat{1}_n \right) \mathcal{L} \hat{\rho}_n(0) \otimes |l\rangle\langle m| \right\}}_{\langle \mathcal{L}_{uv,lm} \rangle_n^0} \\ & + i \sum_{uv \in \{ab\}} \int_0^\tau d\tau' \underbrace{\frac{1}{\hbar} \text{Tr} \left\{ \left( |k\rangle\langle j| \otimes \hat{1}_n \right) \mathcal{L} e^{-i\mathcal{L}(\tau-\tau')/\hbar} \hat{\rho}_n(0) \otimes |u\rangle\langle v| \right\}}_{\mathcal{F}_{jk,uv}(\tau-\tau')} \\ & \quad \times \underbrace{\frac{1}{\hbar^2} \text{Tr} \left\{ \left( |v\rangle\langle u| \otimes \hat{1}_n \right) \mathcal{L} e^{-i\mathcal{Q}^{\text{set}}\mathcal{L}\tau'/\hbar} \mathcal{Q}^{\text{set}} \mathcal{L} \hat{\rho}_n(0) \otimes |l\rangle\langle m| \right\}}_{\mathcal{K}_{uv,lm}^{\text{set}}(\tau')}. \end{aligned}$$

Therefore, the Volterra equation for the subset memory kernel is given by

$$\mathcal{K}_{jk,lm}^{\text{set}}(\tau) = i\dot{\mathcal{F}}_{jk,lm}(\tau) - \frac{1}{\hbar} \sum_{uv \in \{ab\}} \mathcal{F}_{jk,uv}(\tau) \langle \mathcal{L}_{uv,lm} \rangle_n^0 + i \sum_{uv \in \{ab\}} \int_0^\tau d\tau' \mathcal{F}_{jk,uv}(\tau-\tau') \mathcal{K}_{uv,lm}^{\text{set}}(\tau') \quad (\text{S.31})$$

Note that  $\langle \mathcal{L}_{jj,kk} \rangle_n^0 = 0$ .

Since the PFIs can be written in terms of the time evolution operator  $\mathcal{U}(\tau)$ , this means that Eq. (S.31) can be rewritten in terms of the time evolution operator for the reduced electronic density operator:

$$\mathcal{K}_{jk,lm}^{\text{set}}(\tau) = -\ddot{\mathcal{U}}_{jk,lm}(\tau) - \frac{i}{\hbar} \sum_{uv \in \{ab\}} \dot{\mathcal{U}}_{jk,uv}(\tau) \langle \mathcal{L}_{uv,lm} \rangle_n^0 - \sum_{uv \in \{ab\}} \int_0^\tau d\tau' \dot{\mathcal{U}}_{jk,uv}(\tau-\tau') \mathcal{K}_{uv,lm}^{\text{set}}(\tau'). \quad (\text{S.32})$$

Next, we consider the explicit expression for the inhomogeneous term, Eq. (S.23). We

substitute the identity in Eq. (S.26) for  $e^{-i\mathcal{Q}^{\text{set}}\mathcal{L}\tau/\hbar}$ , which yields:

$$I_{jk}^{\text{set}}(t) = -\frac{i}{\hbar} \text{Tr} \left\{ \left( |k\rangle\langle j| \otimes \hat{1}_n \right) \mathcal{L} e^{-i\mathcal{L}t/\hbar} \left[ \hat{\rho}(0) - \sum_{lm \in \{ab\}} \hat{\rho}_n(0) \otimes |l\rangle\langle m| \sigma_{lm}(0) \right] \right\} \\ + \frac{1}{\hbar^2} \int_0^t d\tau \text{Tr} \left\{ \left( |k\rangle\langle j| \otimes \hat{1}_n \right) \mathcal{L} e^{-i\mathcal{L}(t-\tau)/\hbar} \mathcal{P}^{\text{set}} \mathcal{L} e^{-i\mathcal{Q}^{\text{set}}\mathcal{L}\tau/\hbar} \left[ \hat{\rho}(0) - \sum_{lm \in \{ab\}} \hat{\rho}_n(0) \otimes |l\rangle\langle m| \sigma_{lm}(0) \right] \right\}.$$

Splitting the first term into two terms at the minus sign and plugging  $\mathcal{P}^{\text{set}}$  from Eq. (S.14) into the second term leads to Eq. (S.33)

$$I_{jk}^{\text{set}}(t) = \underbrace{-\frac{i}{\hbar} \text{Tr} \left\{ \left( |k\rangle\langle j| \otimes \hat{1}_n \right) \mathcal{L} e^{-i\mathcal{L}t/\hbar} \hat{\rho}(0) \right\}}_{= Z_{jk}(t)} \\ + i \sum_{lm \in \{ab\}} \frac{1}{\hbar} \text{Tr} \left\{ \left( |k\rangle\langle j| \otimes \hat{1}_n \right) \mathcal{L} e^{-i\mathcal{L}t/\hbar} \hat{\rho}_n(0) \otimes |l\rangle\langle m| \right\} \underbrace{\sigma_{lm}(0)}_{= \mathcal{F}_{jk,lm}(t)} \\ + i \sum_{uv \in \{ab\}} \int_0^t d\tau \frac{1}{\hbar} \text{Tr} \left\{ \left( |k\rangle\langle j| \otimes \hat{1}_n \right) \mathcal{L} e^{-i\mathcal{L}(t-\tau)/\hbar} \hat{\rho}_n(0) \otimes |u\rangle\langle v| \right\} \underbrace{= \mathcal{F}_{jk,uv}(t-\tau)} \\ \times \underbrace{\left[ -\frac{i}{\hbar} \text{Tr} \left\{ \left( |\lambda\rangle\langle \lambda| \otimes \hat{1}_n \right) \mathcal{L} e^{-i\mathcal{Q}^{\text{set}}\mathcal{L}\tau/\hbar} \left[ \hat{\rho}(0) - \sum_{lm \in \{ab\}} \hat{\rho}_n(0) \otimes |k\rangle\langle k| \sigma_{kk}(0) \right] \right\} \right]}_{= I_{uv}^{\text{set}}(\tau)} \Bigg]. \\ I_{jk}^{\text{set}}(t) = Z_{jk}(t) + i \sum_{lm \in \{ab\}} \mathcal{F}_{jk,lm}(t) \sigma_{lm}(0) + i \sum_{uv \in \{ab\}} \int_0^t d\tau \mathcal{F}_{jk,uv}(t-\tau) I_{uv}^{\text{set}}(\tau). \quad (\text{S.33})$$

Here,  $\{Z_{jk}(t)\}$  is given by

$$Z_{jk}(t) = -\frac{i}{\hbar} \text{Tr} \left\{ \left( |k\rangle\langle j| \otimes \hat{1}_n \right) \mathcal{L} e^{-i\mathcal{L}t/\hbar} \hat{\rho}(0) \right\}. \quad (\text{S.34})$$

If the overall initial state is of the commonly encountered form  $\hat{\rho}(0) = \hat{\rho}_n(0) \otimes |\alpha\rangle\langle\alpha|$ , then  $Z_{jk}(t)$  is equivalent to  $-i\mathcal{F}_{jk,\alpha\alpha}(t) = \dot{\mathcal{U}}_{jk,\alpha\alpha}(t)$ .

### S.III Equivalence between the TFD Schrödinger equation and the quantum Liouville equation

In this section, we show that when the thermal wavepacket  $|\psi_\gamma(\beta, t)\rangle$  is defined such that

$$\hat{\rho}(t) = \text{Tr}_f \left\{ |\psi_\gamma(\beta, t)\rangle \langle \psi_\gamma(\beta, t)| \right\}, \quad (\text{S.35})$$

and evolves according to the so-called TFD Schrödinger equation:

$$\frac{d}{dt} |\psi_\gamma(\beta, t)\rangle = -\frac{i}{\hbar} \bar{H} |\psi_\gamma(\beta, t)\rangle, \quad (\text{S.36})$$

where  $\bar{H} = \hat{H} \otimes \tilde{1}_n$ , then  $\hat{\rho}(t)$  correctly evolves according to the quantum Liouville equation.

To see this, take the time derivative on both sides of Eq. (S.35), we obtain:

$$\frac{d}{dt} \hat{\rho}(t) = \text{Tr}_f \left[ \left( \frac{d}{dt} |\psi_\gamma(\beta, t)\rangle \right) \langle \psi_\gamma(\beta, t)| + |\psi_\gamma(\beta, t)\rangle \left( \frac{d}{dt} \langle \psi_\gamma(\beta, t)| \right) \right]. \quad (\text{S.37})$$

Plugging Eq. (S.36) into the right hand side of Eq. (S.37), we obtain:

$$\frac{d}{dt} \hat{\rho}(t) = \text{Tr}_f \left[ -\frac{i}{\hbar} (\hat{H} \otimes \tilde{1}_n) |\psi_\gamma(\beta, t)\rangle \langle \psi_\gamma(\beta, t)| + |\psi_\gamma(\beta, t)\rangle \langle \psi_\gamma(\beta, t)| \frac{i}{\hbar} (\hat{H} \otimes \tilde{1}_n) \right]. \quad (\text{S.38})$$

Pulling  $\hat{H}$  out of the partial trace with  $\text{Tr}_f[(\hat{H} \otimes \tilde{1}_n) \bar{B}] = \hat{H} \text{Tr}_f[\bar{B}]$  for any double space operator  $\bar{B}$ ,

$$\begin{aligned} \frac{d}{dt} \hat{\rho}(t) &= -\frac{i}{\hbar} \hat{H} \text{Tr}_f[|\psi_\gamma(\beta, t)\rangle \langle \psi_\gamma(\beta, t)|] + \text{Tr}_f[|\psi_\gamma(\beta, t)\rangle \langle \psi_\gamma(\beta, t)|] \frac{i}{\hbar} \hat{H} \\ &= -\frac{i}{\hbar} [\hat{H}, \hat{\rho}(t)], \end{aligned} \quad (\text{S.39})$$

which is the quantum Liouville equation.

### S.IV Linear Combinations for Off-Diagonal Initial States of $\mathcal{U}(t)$

The TT-TFD method requires the initial electronic state to be in a pure state, e.g.,  $|\gamma\rangle\langle\gamma|$ . However, in order to obtain the time evolution operator of the electronic reduced density matrix,  $\mathcal{U}(t)$ , necessary for obtaining the PFIs, we need to start in off-diagonal initial states, e.g.,  $\hat{\sigma}(0) = |u\rangle\langle v|$  when  $u \neq v$ . This problem can be bypassed by starting in a set of pure states and using linear combinations to calculate the off-diagonal initial states. The choice of the set of initial states

is not unique but a relatively unbiased choice is

$$\begin{aligned}\hat{X}_{uv} &= \frac{1}{2} \left[ |u\rangle\langle u| + |v\rangle\langle v| + |u\rangle\langle v| + |v\rangle\langle u| \right] , \\ \hat{Y}_{uv} &= \frac{1}{2} \left[ |u\rangle\langle u| + |v\rangle\langle v| - i|u\rangle\langle v| + i|v\rangle\langle u| \right] .\end{aligned}\tag{S.40}$$

This choice is also used in Ref. 6 for PFIs obtained from the Ehrenfest method.

In practice, one starts with  $\hat{X}_{uv}$  and  $\hat{Y}_{uv}$  instead of  $|u\rangle\langle v|$  and  $|v\rangle\langle u|$  as initial electronic states, to obtain the TT-TFD calculations of

$$\langle \psi_{\theta,jj\hat{X}_{uv}}(t) | \psi_{\theta,jk\hat{X}_{uv}}(t) \rangle , \quad \langle \psi_{\theta,jj\hat{Y}_{uv}}(t) | \psi_{\theta,jk\hat{Y}_{uv}}(t) \rangle .\tag{S.41}$$

The corresponding results for  $|u\rangle\langle v|$  and  $|v\rangle\langle u|$  as the initial electronic states can then be expressed as linear combinations of the results in Eq. (S.41). More specifically,

$$\begin{aligned}\mathcal{U}_{jk,uv}(t) &= \langle \psi_{\theta,jj\hat{X}_{uv}}(t) | \psi_{\theta,jk\hat{X}_{uv}}(t) \rangle + i \langle \psi_{\theta,jj\hat{Y}_{uv}}(t) | \psi_{\theta,jk\hat{Y}_{uv}}(t) \rangle \\ &\quad - \frac{1}{2}(1+i) \left[ \langle \psi_{\theta,jj\hat{X}_{uv}}(t) | \psi_{\theta,jk\hat{X}_{uv}}(t) \rangle - \langle \psi_{\theta,jj\hat{Y}_{uv}}(t) | \psi_{\theta,jk\hat{Y}_{uv}}(t) \rangle \right],\end{aligned}\tag{S.42}$$

$$\begin{aligned}\mathcal{U}_{jk,vu}(t) &= \langle \psi_{\theta,jj\hat{X}_{uv}}(t) | \psi_{\theta,jk\hat{X}_{uv}}(t) \rangle - i \langle \psi_{\theta,jj\hat{Y}_{uv}}(t) | \psi_{\theta,jk\hat{Y}_{uv}}(t) \rangle \\ &\quad - \frac{1}{2}(1-i) \left[ \langle \psi_{\theta,jj\hat{X}_{uv}}(t) | \psi_{\theta,jk\hat{X}_{uv}}(t) \rangle - \langle \psi_{\theta,jj\hat{Y}_{uv}}(t) | \psi_{\theta,jk\hat{Y}_{uv}}(t) \rangle \right].\end{aligned}\tag{S.43}$$

## S.V Graphs of the Projection-Free Inputs

Given in this section are the graphs of the imaginary part of  $\mathcal{F}(\tau)$  and the real and imaginary parts of  $\dot{\mathcal{F}}(\tau)$  for models 1, 2, 3, and 6. The real part of  $\mathcal{F}(\tau)$  is not show because it is zero for all models for both TT-TFD and LSCII.

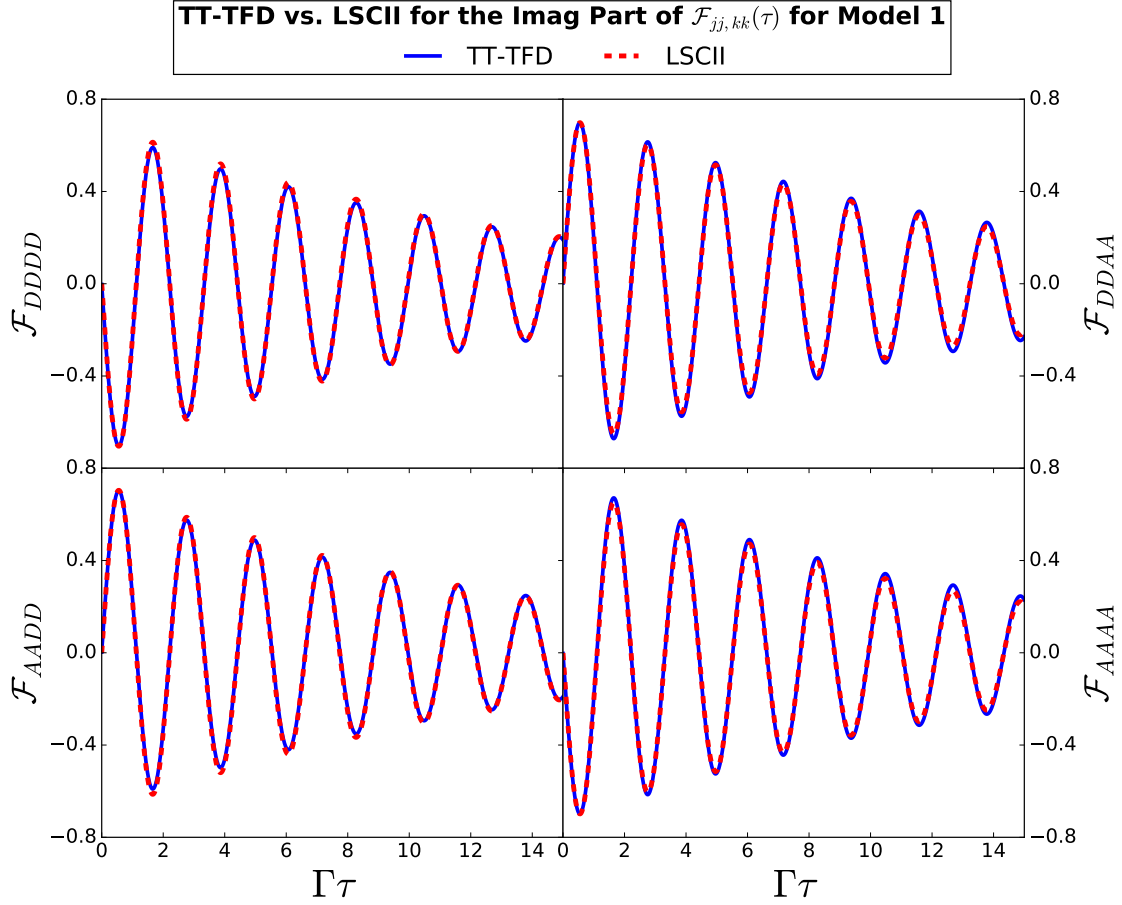

Figure S1: Imaginary parts of the  $DDDD$ ,  $DDAA$ ,  $AADD$  and  $AAAA$  matrix elements of  $\mathcal{F}(\tau)$  for model 1, as obtained via TT-TFD (solid blue lines) and LSCII (dashed red lines).

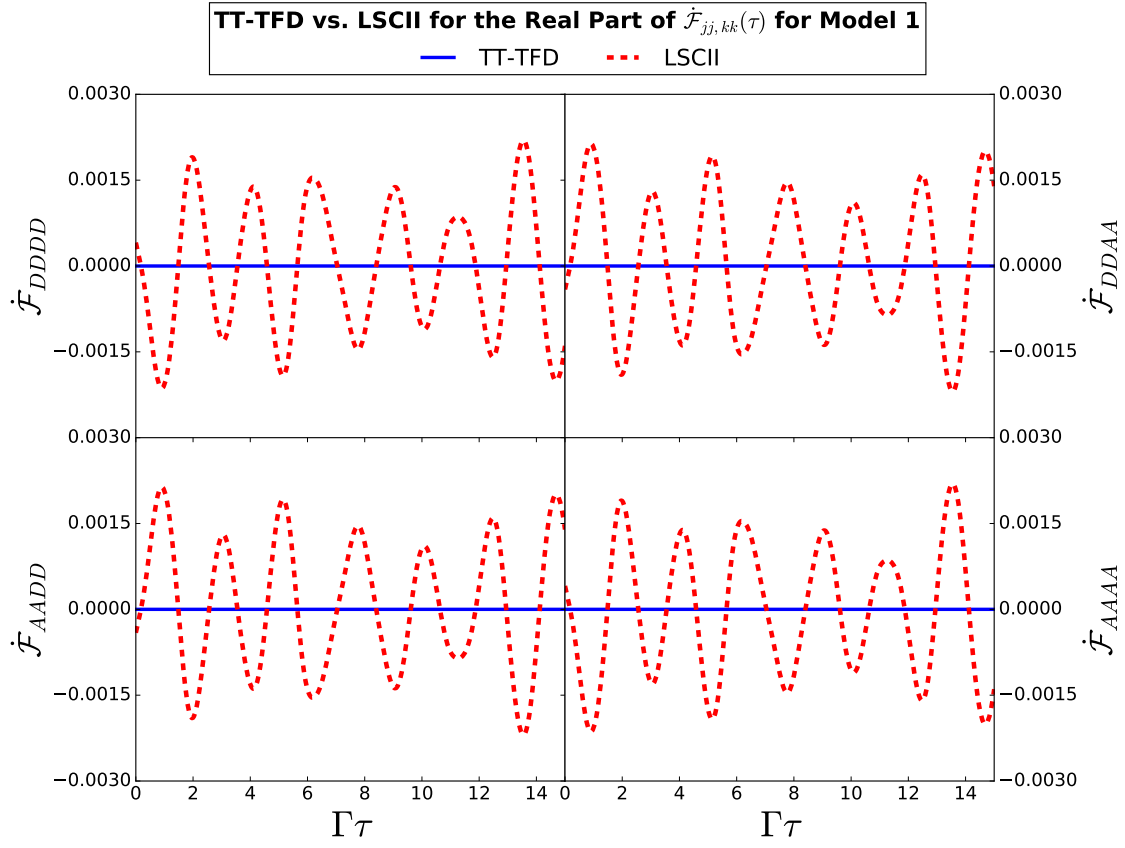

Figure S2: Real parts of the  $DDDD$ ,  $DDAA$ ,  $AADD$  and  $AAAA$  matrix elements of  $\dot{\mathcal{F}}(\tau)$  for model 1, as obtained via TT-TFD (solid blue lines) and LSCII (dashed red lines).

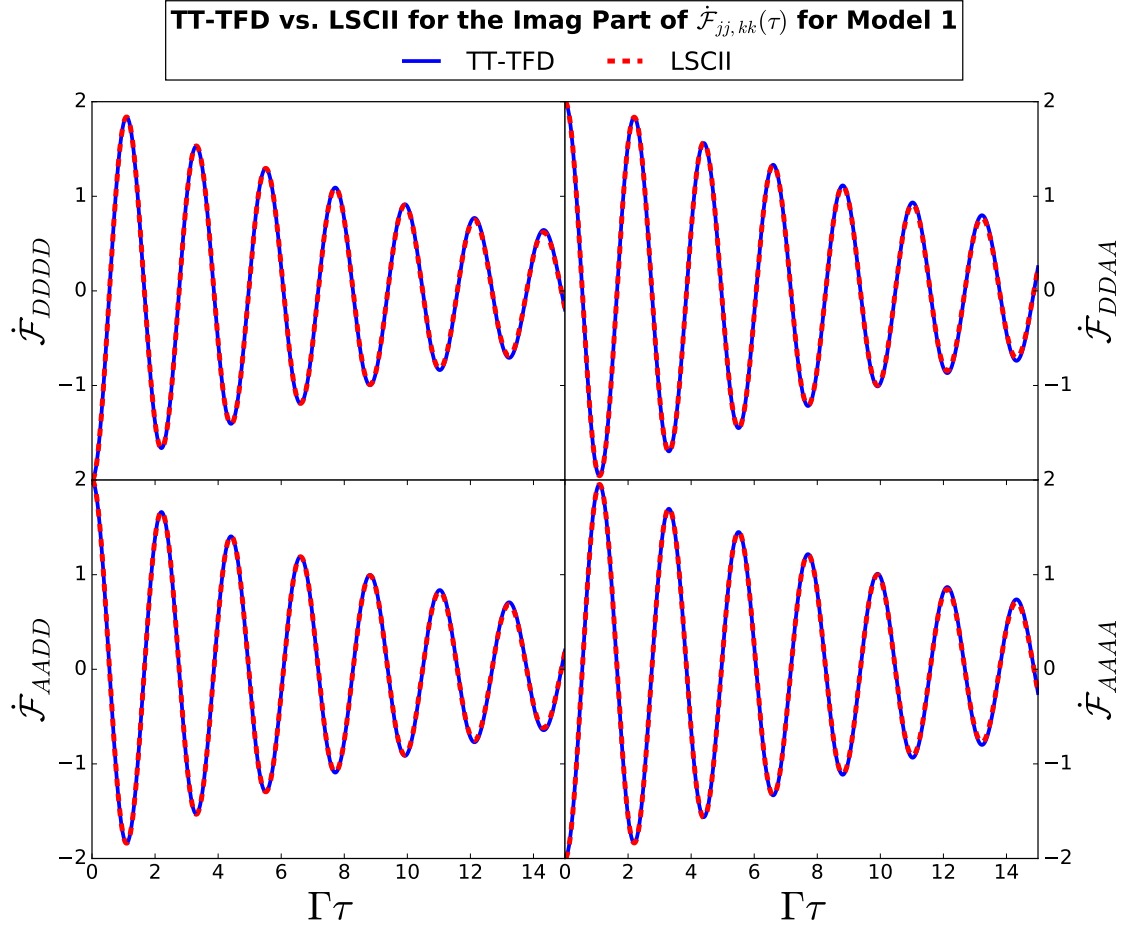

Figure S3: Imaginary parts of the  $DDDD$ ,  $DDAA$ ,  $AADD$  and  $AAAA$  matrix elements of  $\dot{\mathcal{F}}(\tau)$  for model 1, as obtained via TT-TFD (solid blue lines) and LSCII (dashed red lines).

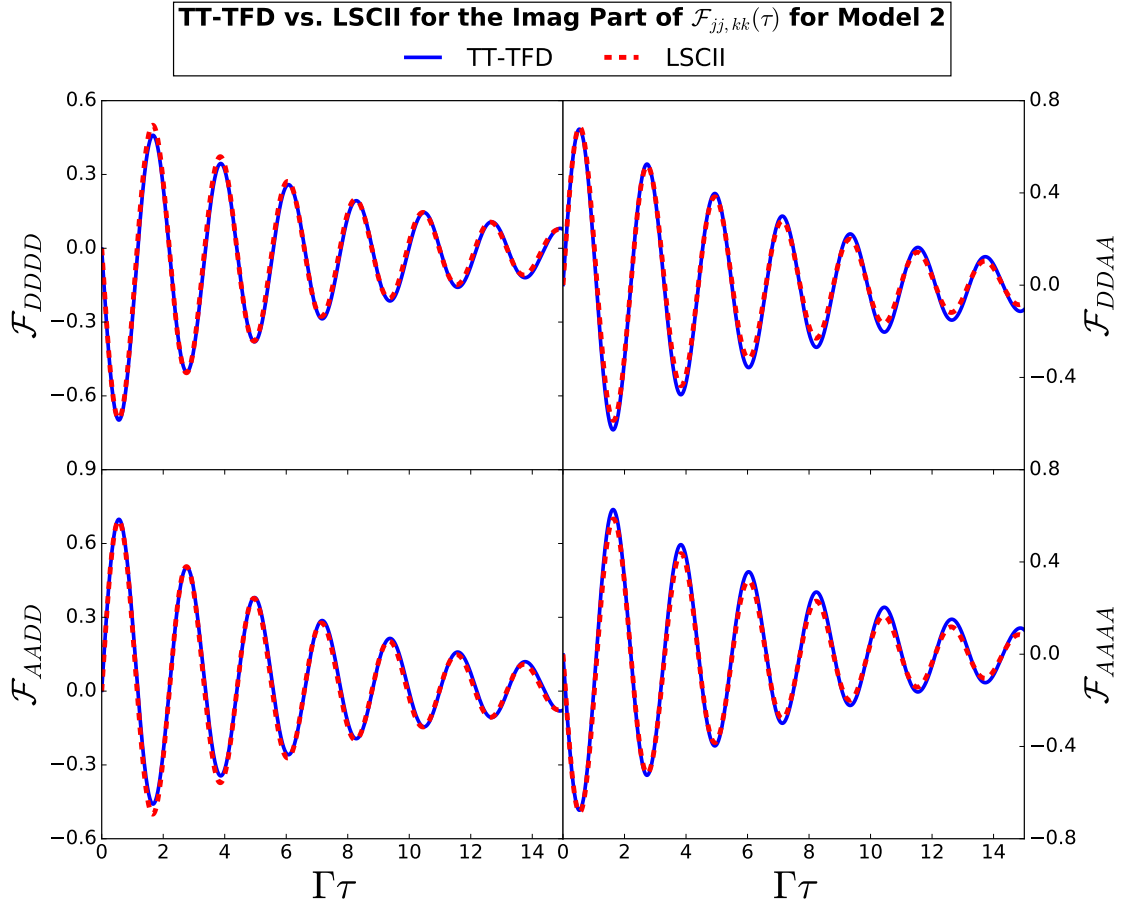

Figure S4: Imaginary parts of the  $DDDD$ ,  $DDAA$ ,  $AADD$  and  $AAAA$  matrix elements of  $\mathcal{F}(\tau)$  for model 2, as obtained via TT-TFD (solid blue lines) and LSCII (dashed red lines).

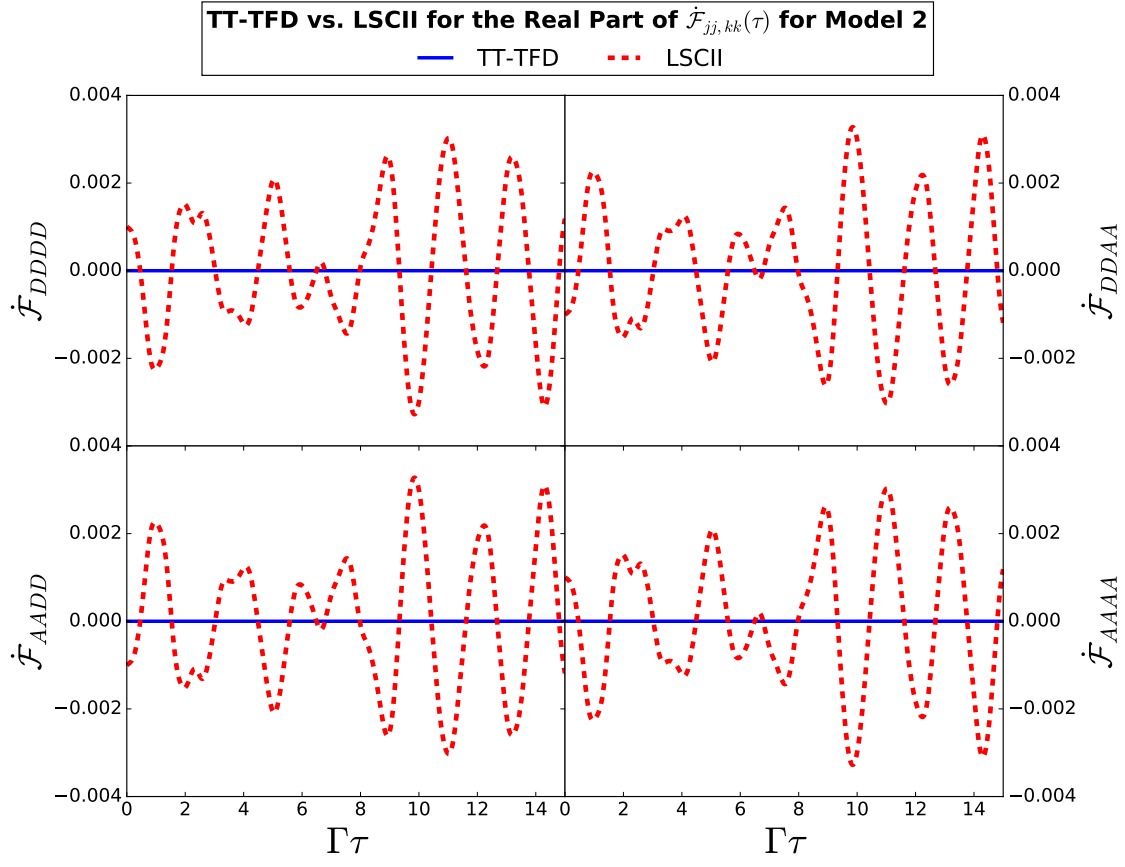

Figure S5: Real parts of the  $DDDD$ ,  $DDAA$ ,  $AADD$  and  $AAAA$  matrix elements of  $\dot{\mathcal{F}}(\tau)$  for model 2, as obtained via TT-TFD (solid blue lines) and LSCII (dashed red lines).

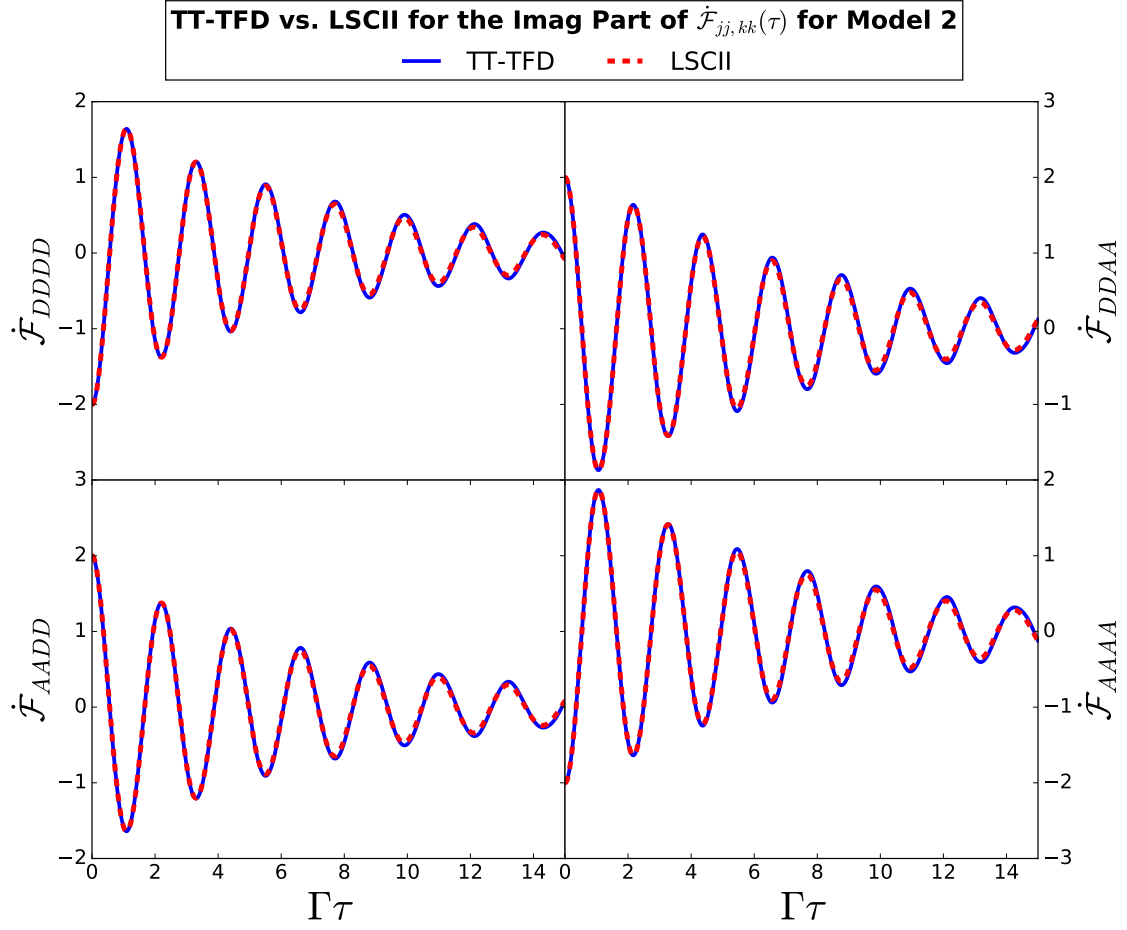

Figure S6: Imaginary parts of the  $DDDD$ ,  $DDAA$ ,  $AADD$  and  $AAAA$  matrix elements of  $\dot{\mathcal{F}}(\tau)$  for model 2, as obtained via TT-TFD (solid blue lines) and LSCII (dashed red lines).

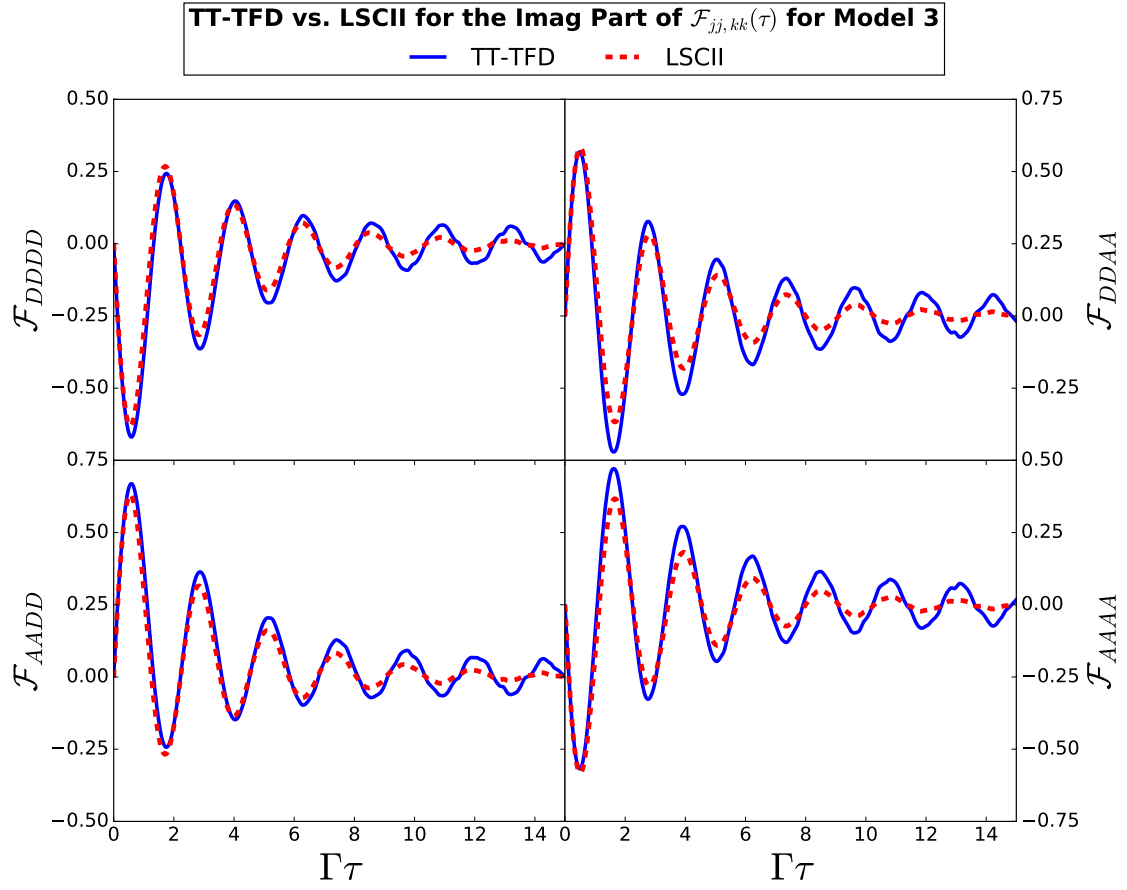

Figure S7: Imaginary parts of the  $DDDD$ ,  $DDAA$ ,  $AADD$  and  $AAAA$  matrix elements of  $\mathcal{F}(\tau)$  for model 3, as obtained via TT-TFD (solid blue lines) and LSCII (dashed red lines).

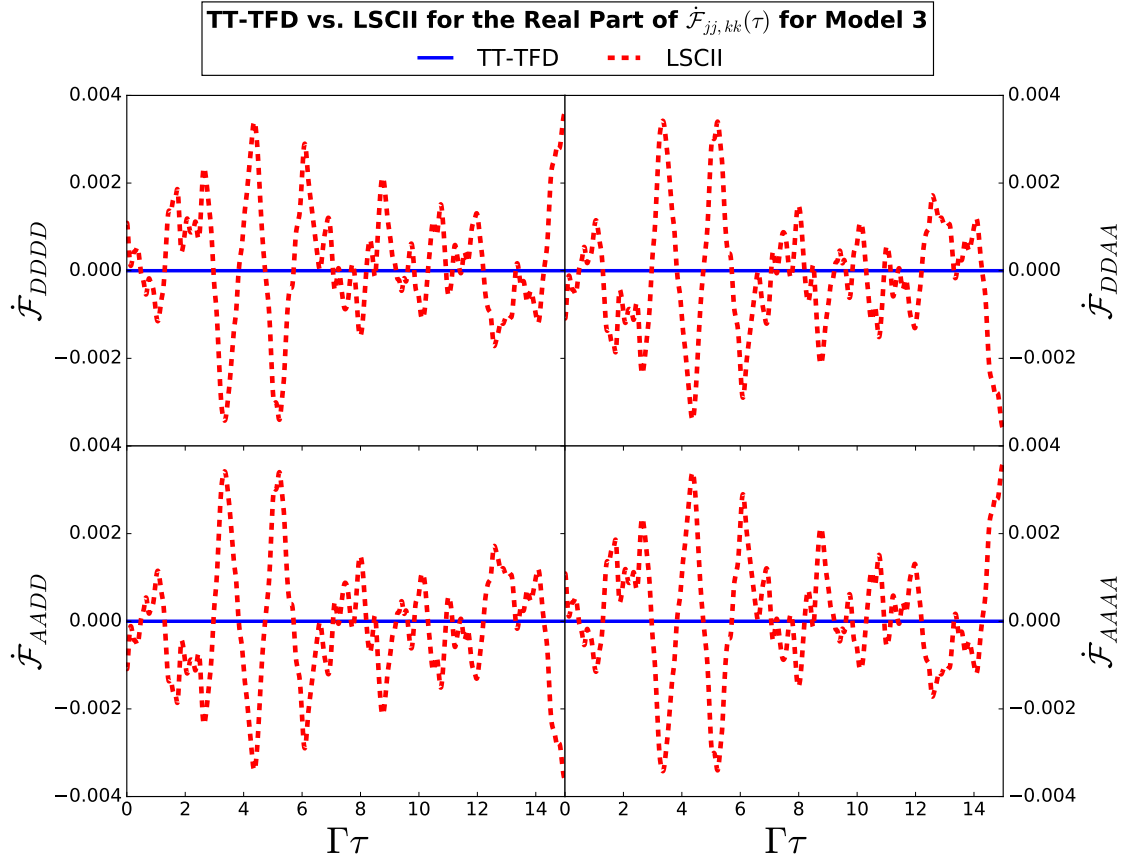

Figure S8: Real parts of the  $DDDD$ ,  $DDAA$ ,  $AADD$  and  $AAAA$  matrix elements of  $\dot{\mathcal{F}}(\tau)$  for model 3, as obtained via TT-TFD (solid blue lines) and LSCII (dashed red lines).

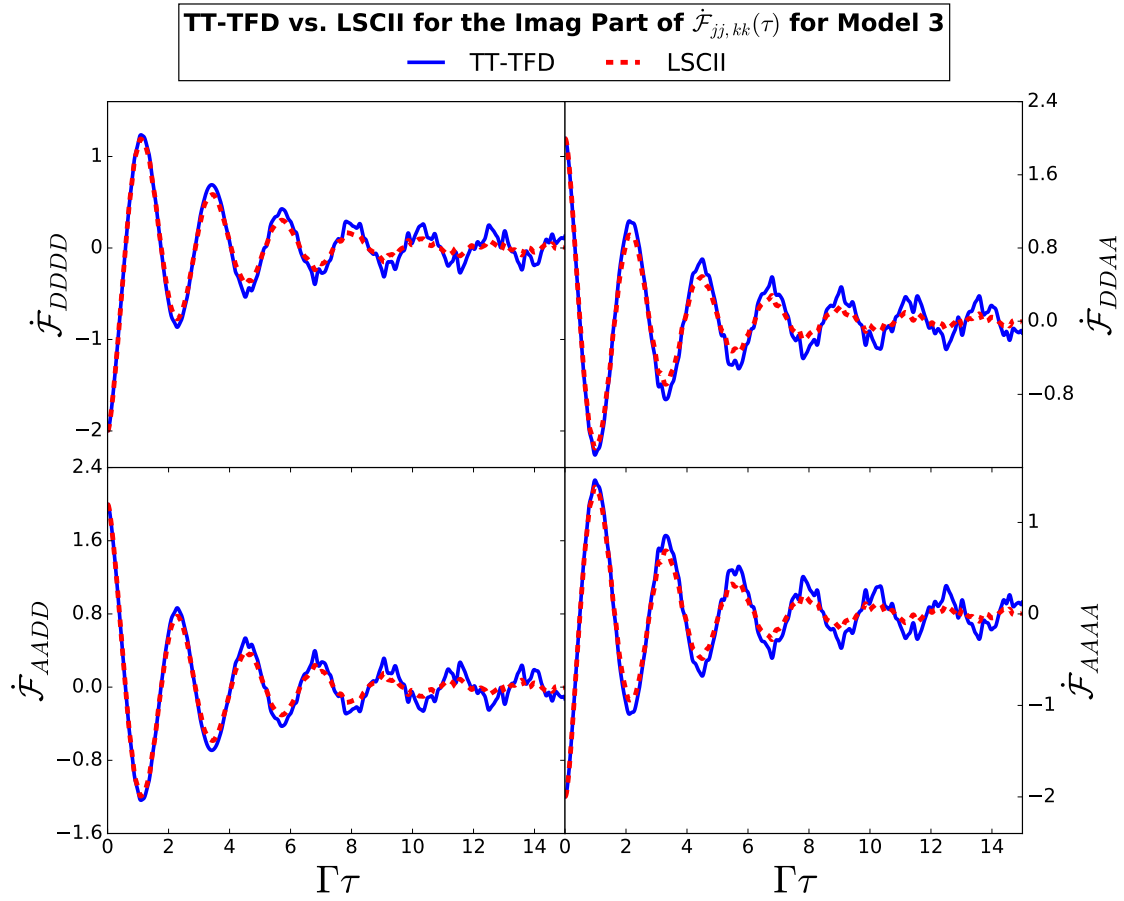

Figure S9: Imaginary parts of the  $DDDD$ ,  $DDAA$ ,  $AADD$  and  $AAAA$  matrix elements of  $\dot{\mathcal{F}}(\tau)$  for model 3, as obtained via TT-TFD (solid blue lines) and LSCII (dashed red lines).

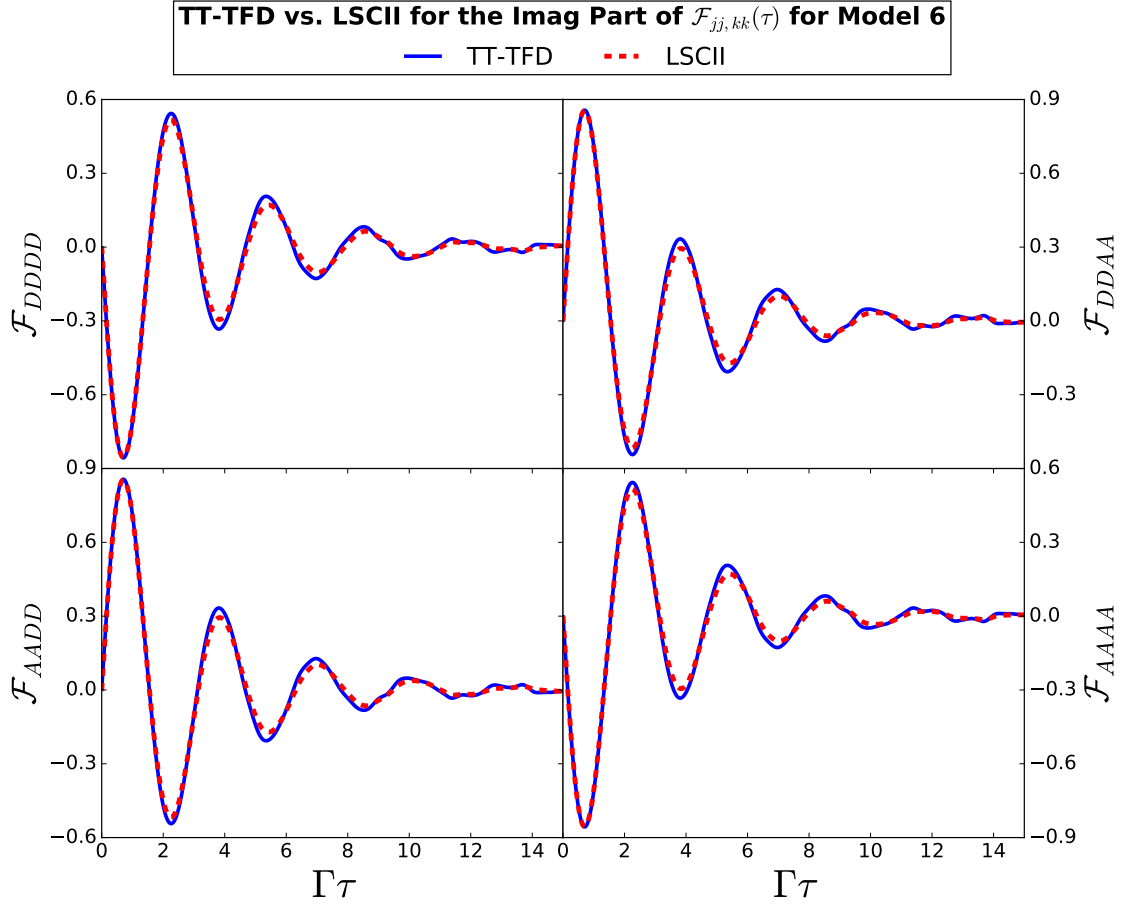

Figure S10: Imaginary parts of the  $DDDD$ ,  $DDAA$ ,  $AADD$  and  $AAAA$  matrix elements of  $\mathcal{F}(\tau)$  for model 6, as obtained via TT-TFD (solid blue lines) and LSCII (dashed red lines).

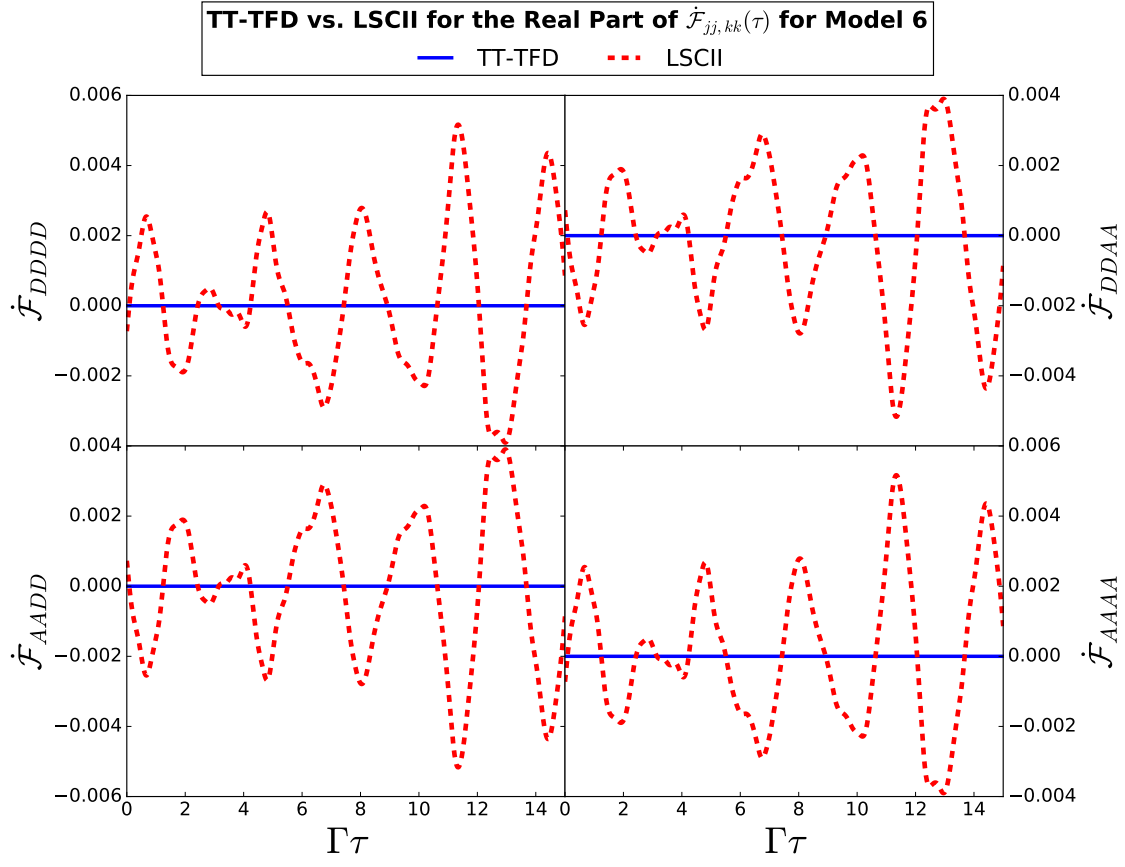

Figure S11: Real parts of the  $DDDD$ ,  $DDAA$ ,  $AADD$  and  $AAAA$  matrix elements of  $\dot{\mathcal{F}}(\tau)$  for model 6, as obtained via TT-TFD (solid blue lines) and LSCII (dashed red lines).

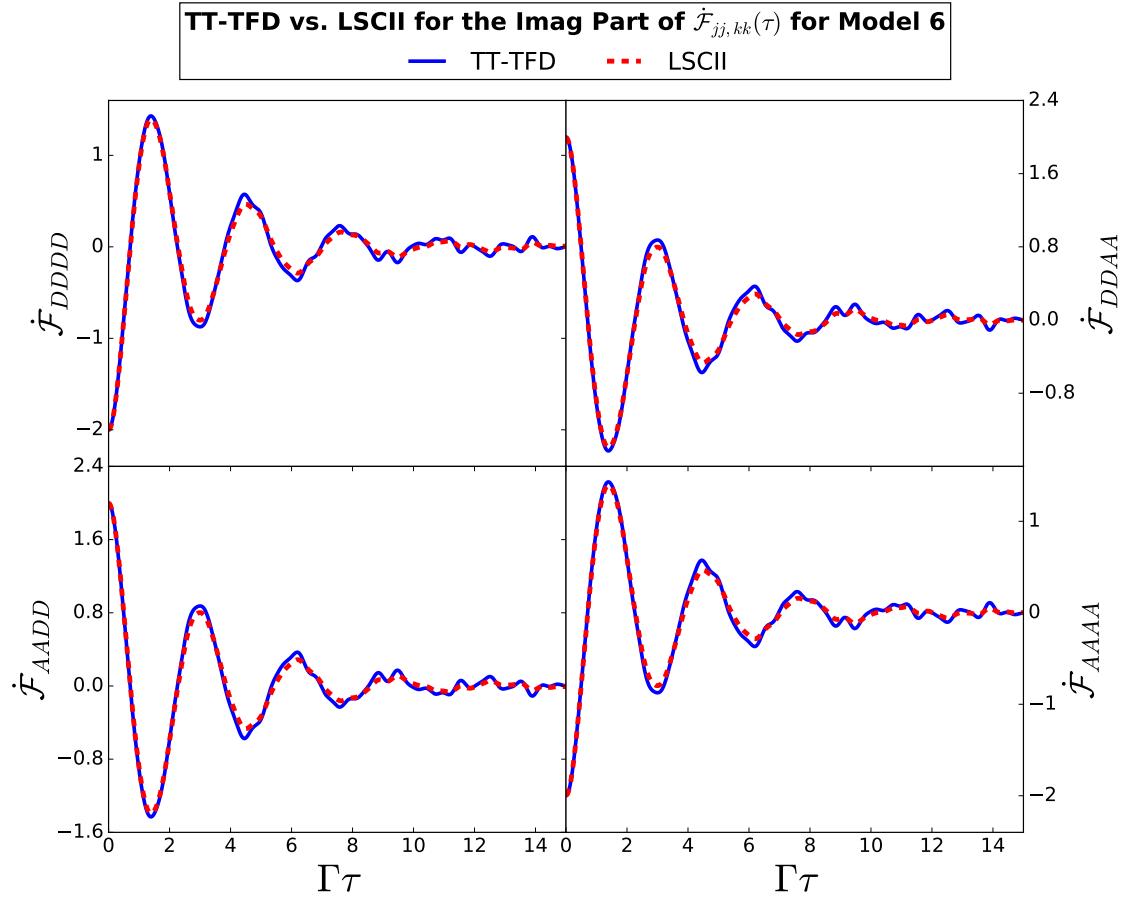

Figure S12: Imaginary parts of the  $DDDD$ ,  $DDAA$ ,  $AADD$  and  $AAAA$  matrix elements of  $\dot{\mathcal{F}}(\tau)$  for model 6, as obtained via TT-TFD (solid blue lines) and LSCII (dashed red lines).

## S.VI Graphs of the Memory Kernels

Given in this section are the graphs of the real and imaginary parts of the memory kernels for models 1, 2, 3, and 6.

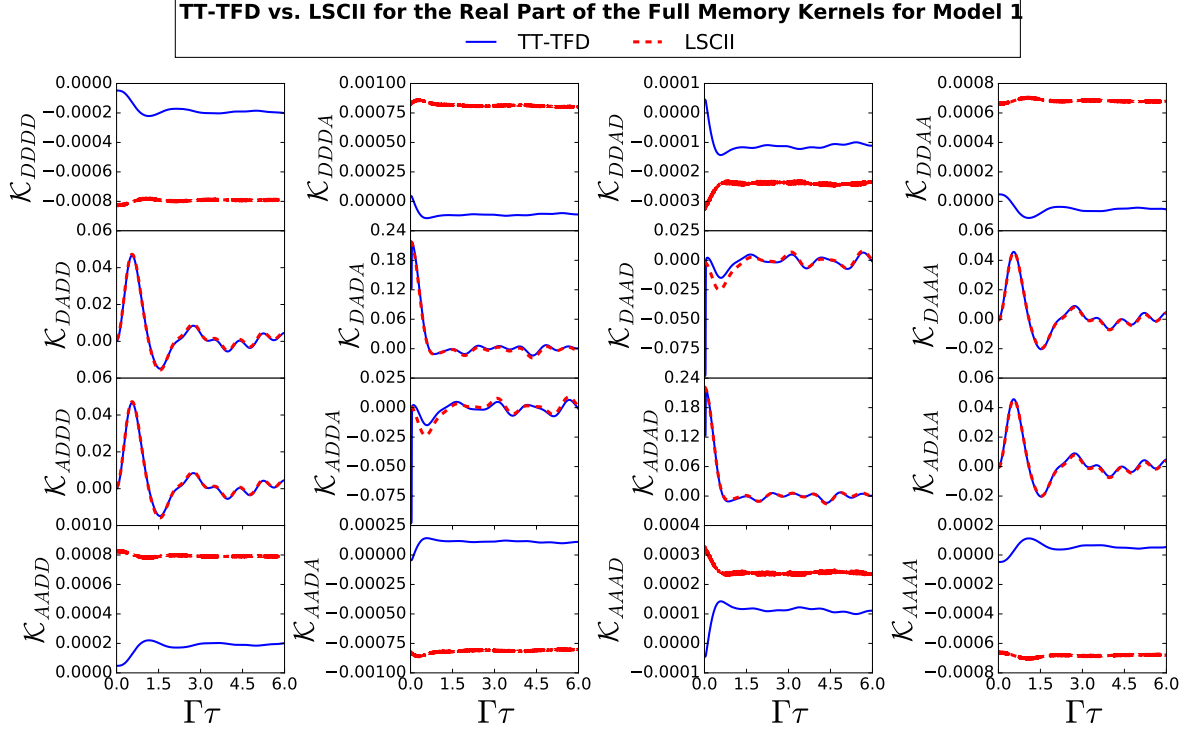

Figure S13: Real parts of the matrix elements of the memory kernel of the GQME for the full electronic density matrix  $[\mathcal{K}^{\text{full}}(\tau)]$  for model 1 as obtained from TT-TFD-based PFIs (solid blue lines) and LSCII-based PFIs (dashed red lines).

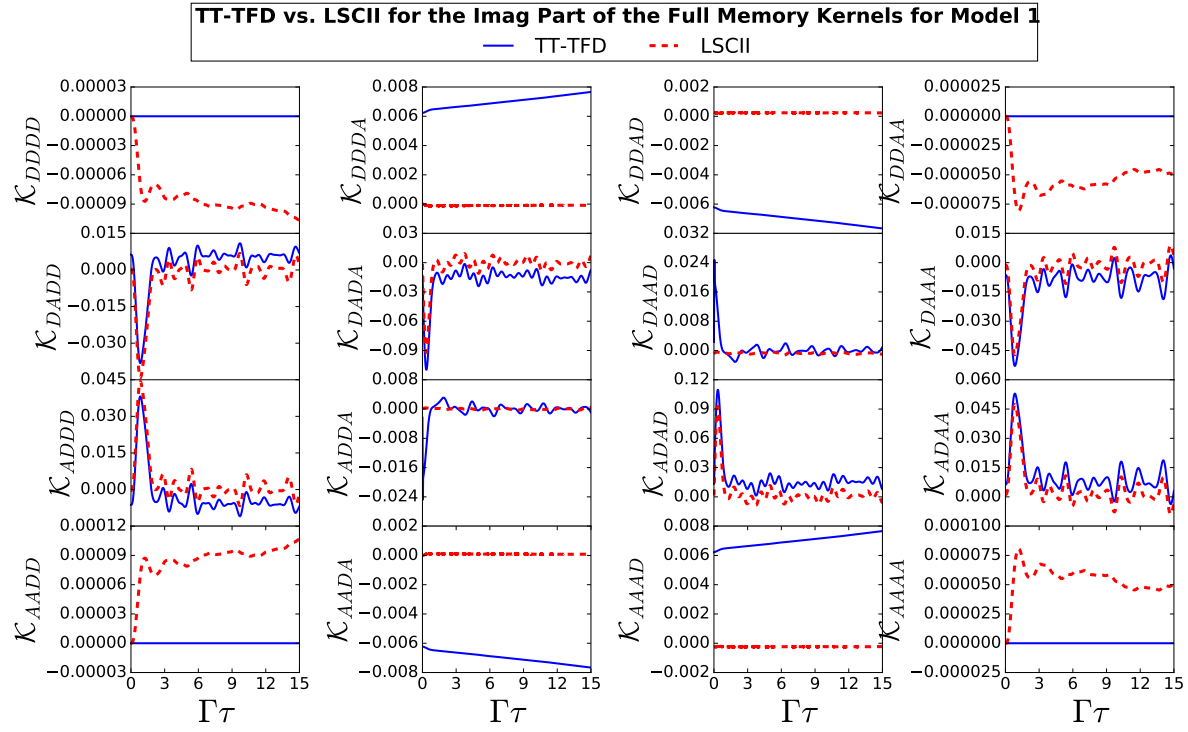

Figure S14: Imaginary parts of the matrix elements of the memory kernel of the GQME for the full electronic density matrix  $[\mathcal{K}^{\text{full}}(\tau)]$  for model 1 as obtained from TT-TFD-based PFIs (solid blue lines) and LSCII-based PFIs (dashed red lines).

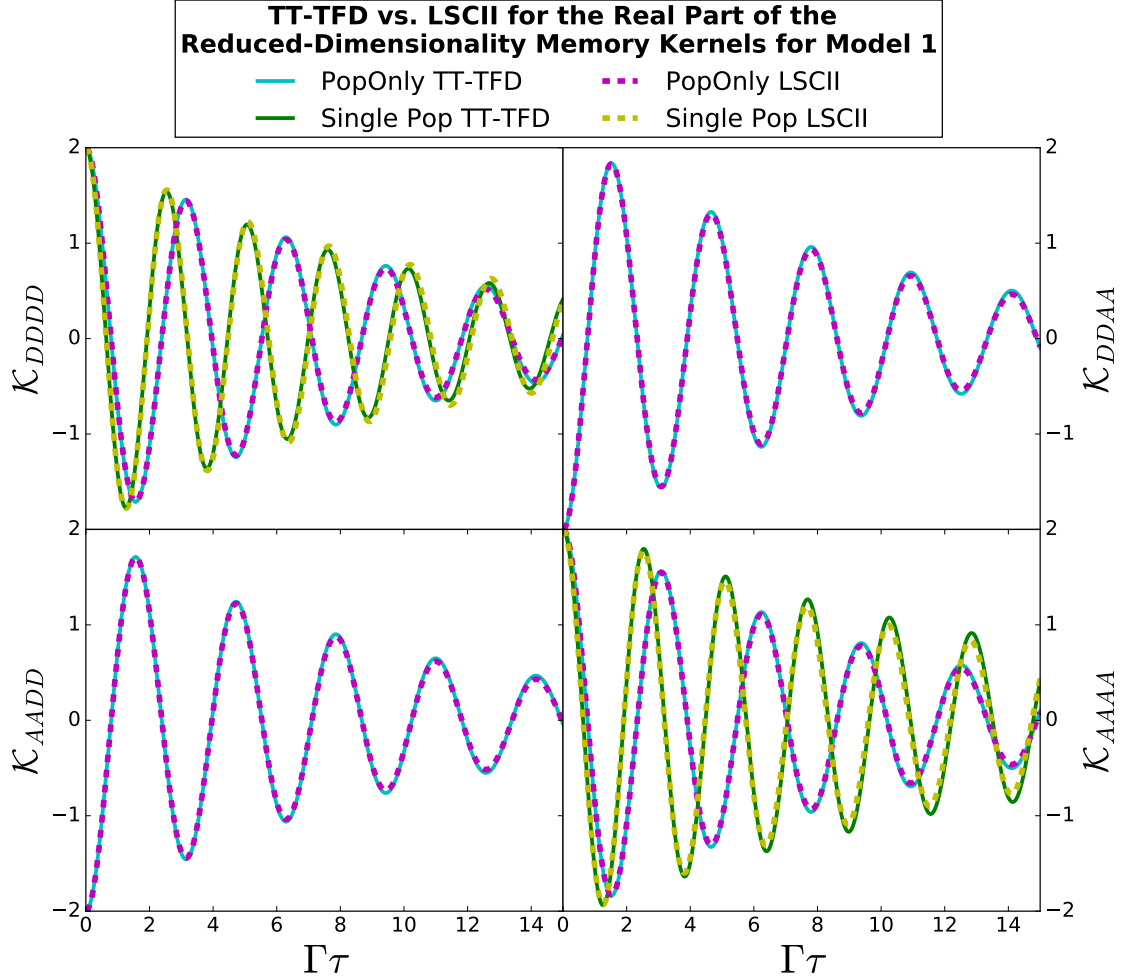

Figure S15: The real parts of the matrix elements of the memory kernels for the populations-only and single-population GQMEs for model 1 as obtained from TT-TFD-based PFIs and LSCII-based PFIs. Shown are the matrix elements of three different memory kernels: (1) The memory kernel of the populations-only GQME [ $\mathcal{K}^{\text{pop}}(\tau)$ ], which has four elements ( $DDDD, DDAA, AADD, AAAA$ ) and is depicted with solid cyan lines for the results from TT-TFD-based PFIs and dashed magenta lines for the results from LSCII-based PFIs; (2) and (3) The single-element memory kernels of the scalar single-population GQMEs [ $\mathcal{K}_{DD,DD}^{\text{donor}}(\tau)$  and  $\mathcal{K}_{AA,AA}^{\text{acceptor}}(\tau)$ ], which are depicted in the  $DDDD$  and  $AAAA$  panels, respectively, with solid green lines for the results from TT-TFD-based PFIs and dashed yellow lines for the results from LSCII-based PFIs.

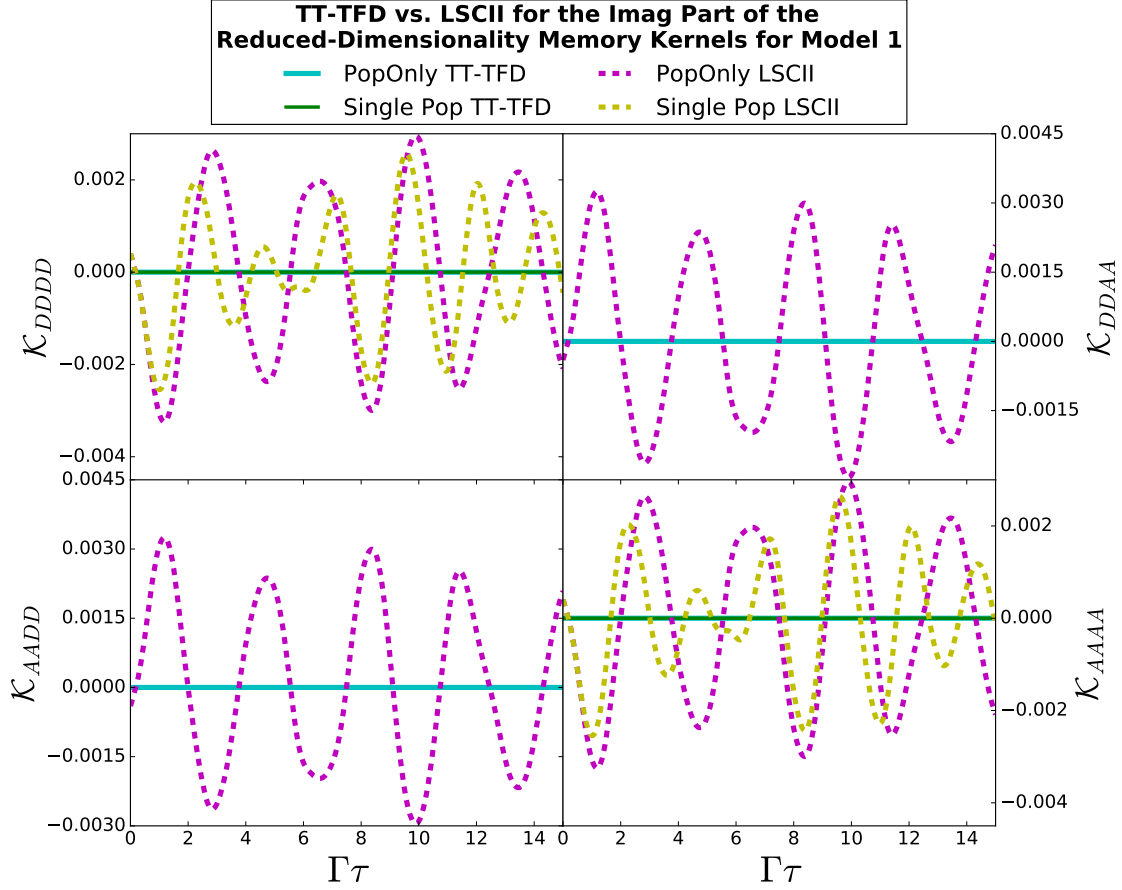

Figure S16: The imaginary parts of the matrix elements of the memory kernels for the populations-only and single-population GQMEs for model 1 as obtained from TT-TFD-based PFIs and LSCII-based PFIs. Shown are the matrix elements of three different memory kernels: (1) The memory kernel of the populations-only GQME [ $\mathcal{K}^{\text{pop}}(\tau)$ ], which has four elements ( $DDDD, DDAA, AADD, AAAA$ ) and is depicted with solid cyan lines for the results from TT-TFD-based PFIs and dashed magenta lines for the results from LSCII-based PFIs; (2) and (3) The single-element memory kernels of the scalar single-population GQMEs [ $\mathcal{K}_{DD,DD}^{\text{donor}}(\tau)$  and  $\mathcal{K}_{AA,AA}^{\text{acceptor}}(\tau)$ ], which are depicted in the  $DDDD$  and  $AAAA$  panels, respectively, with solid green lines for the results from TT-TFD-based PFIs and dashed yellow lines for the results from LSCII-based PFIs.

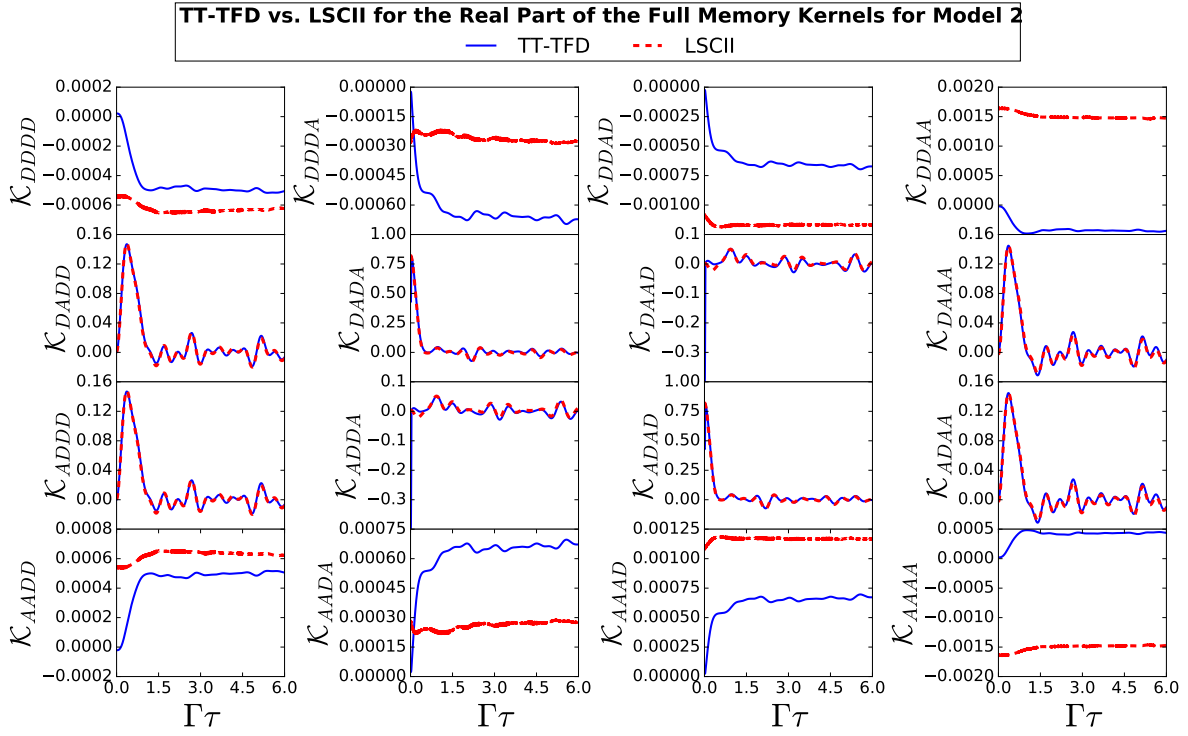

Figure S17: Real parts of the matrix elements of the memory kernel of the GQME for the full electronic density matrix  $[\mathcal{K}^{\text{full}}(\tau)]$  for model 2 as obtained from TT-TFD-based PFIs (solid blue lines) and LSCII-based PFIs (dashed red lines).

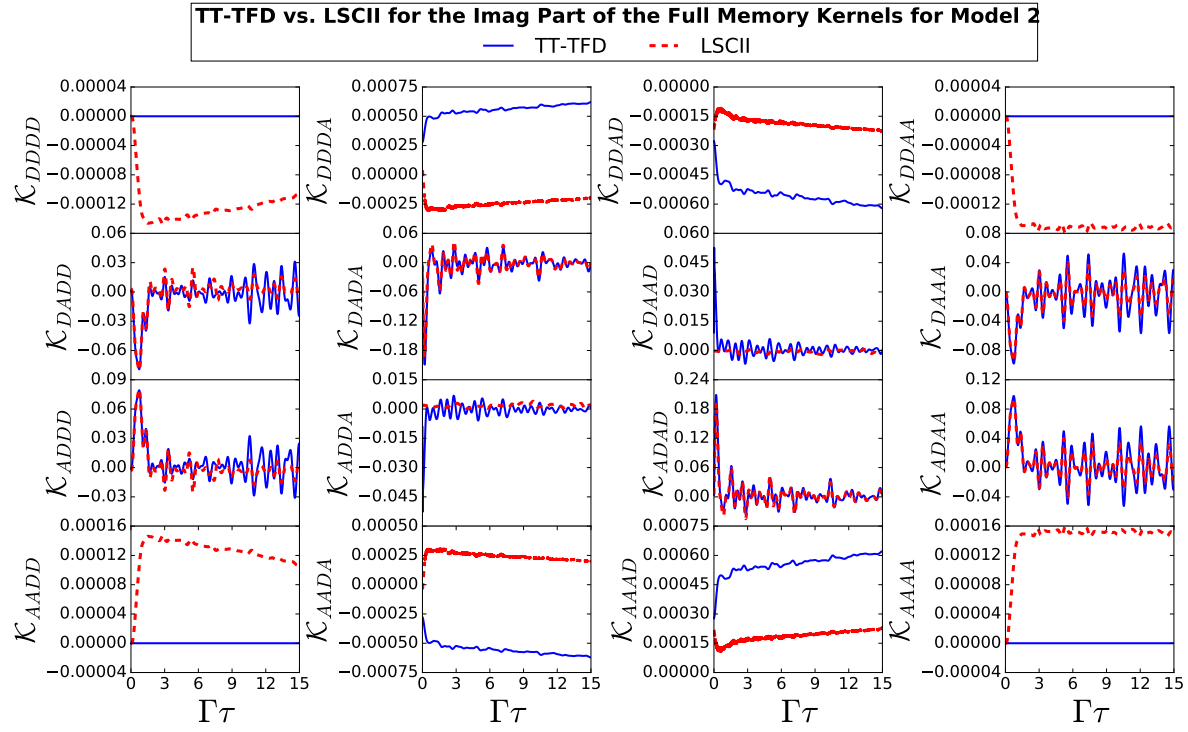

Figure S18: Imaginary parts of the matrix elements of the memory kernel of the GQME for the full electronic density matrix  $[\mathcal{K}^{\text{full}}(\tau)]$  for model 2 as obtained from TT-TFD-based PFIs (solid blue lines) and LSCII-based PFIs (dashed red lines).

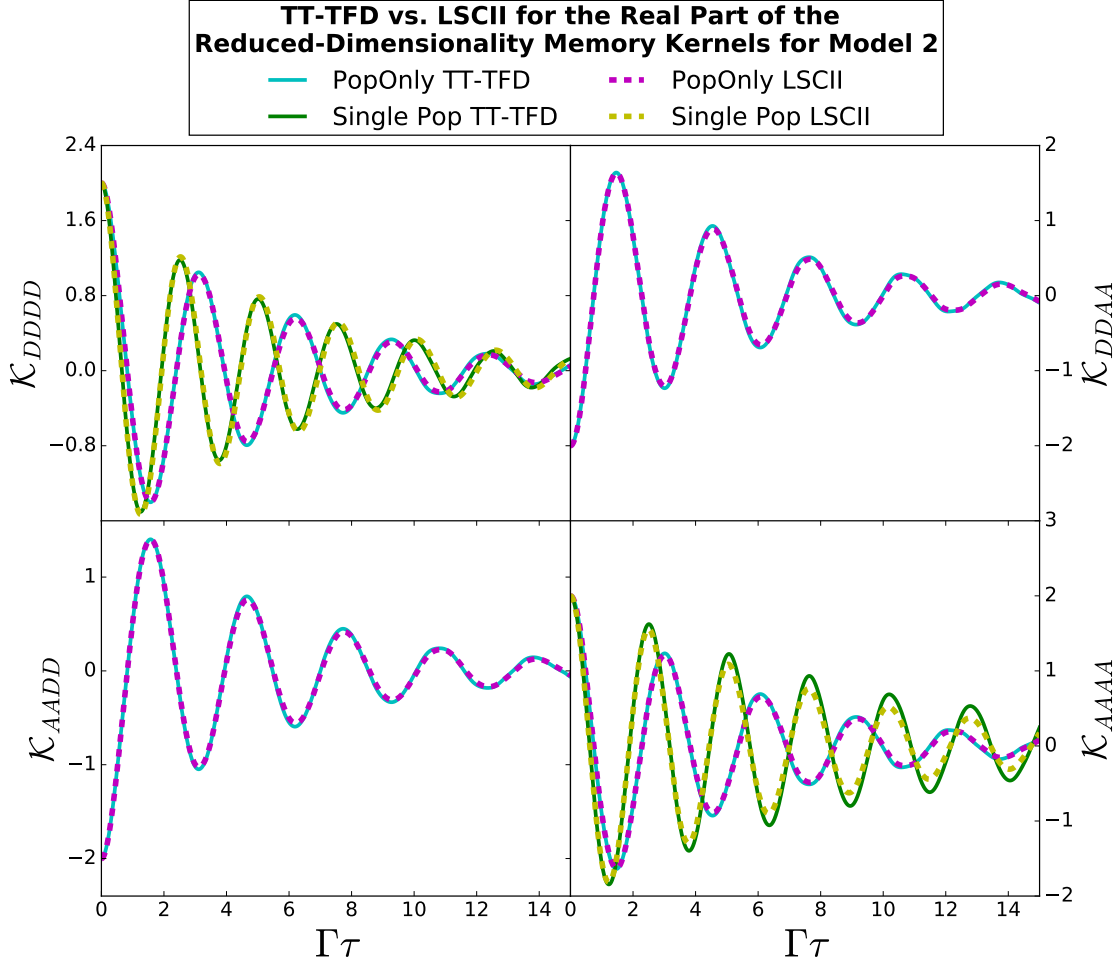

Figure S19: The real parts of the matrix elements of the memory kernels for the populations-only and single-population GQMEs for model 2 as obtained from TT-TFD-based PFIs and LSCII-based PFIs. Shown are the matrix elements of three different memory kernels: (1) The memory kernel of the populations-only GQME [ $\mathcal{K}^{\text{pop}}(\tau)$ ], which has four elements ( $DDDD, DDAA, AADD, AAAA$ ) and is depicted with solid cyan lines for the results from TT-TFD-based PFIs and dashed magenta lines for the results from LSCII-based PFIs; (2) and (3) The single-element memory kernels of the scalar single-population GQMEs [ $\mathcal{K}_{DD,DD}^{\text{donor}}(\tau)$  and  $\mathcal{K}_{AA,AA}^{\text{acceptor}}(\tau)$ ], which are depicted in the  $DDDD$  and  $AAAA$  panels, respectively, with solid green lines for the results from TT-TFD-based PFIs and dashed yellow lines for the results from LSCII-based PFIs.

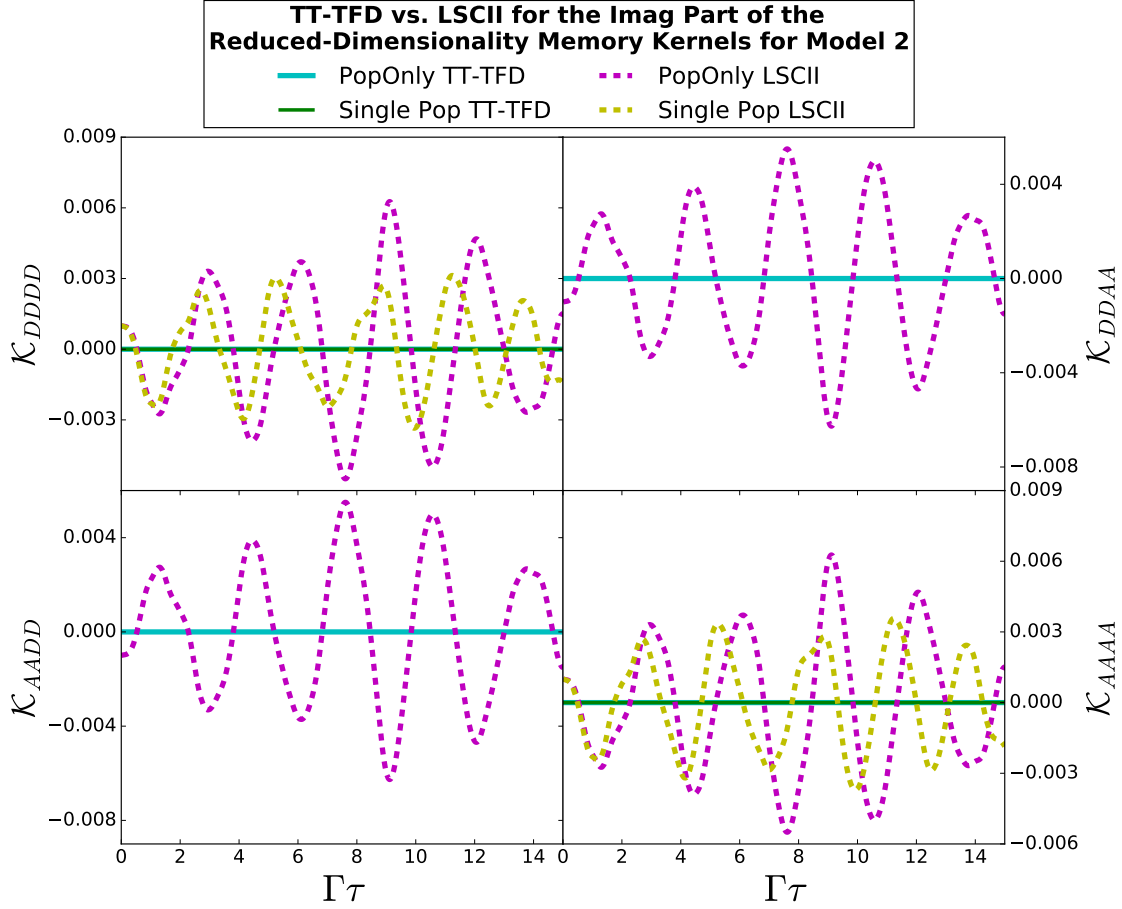

Figure S20: The imaginary parts of the matrix elements of the memory kernels for the populations-only and single-population GQMEs for model 2 as obtained from TT-TFD-based PFIs and LSCII-based PFIs. Shown are the matrix elements of three different memory kernels: (1) The memory kernel of the populations-only GQME [ $\mathcal{K}^{\text{pop}}(\tau)$ ], which has four elements ( $DDDD, DDAA, AADD, AAAA$ ) and is depicted with solid cyan lines for the results from TT-TFD-based PFIs and dashed magenta lines for the results from LSCII-based PFIs; (2) and (3) The single-element memory kernels of the scalar single-population GQMEs [ $\mathcal{K}_{DD,DD}^{\text{donor}}(\tau)$  and  $\mathcal{K}_{AA,AA}^{\text{acceptor}}(\tau)$ ], which are depicted in the  $DDDD$  and  $AAAA$  panels, respectively, with solid green lines for the results from TT-TFD-based PFIs and dashed yellow lines for the results from LSCII-based PFIs.

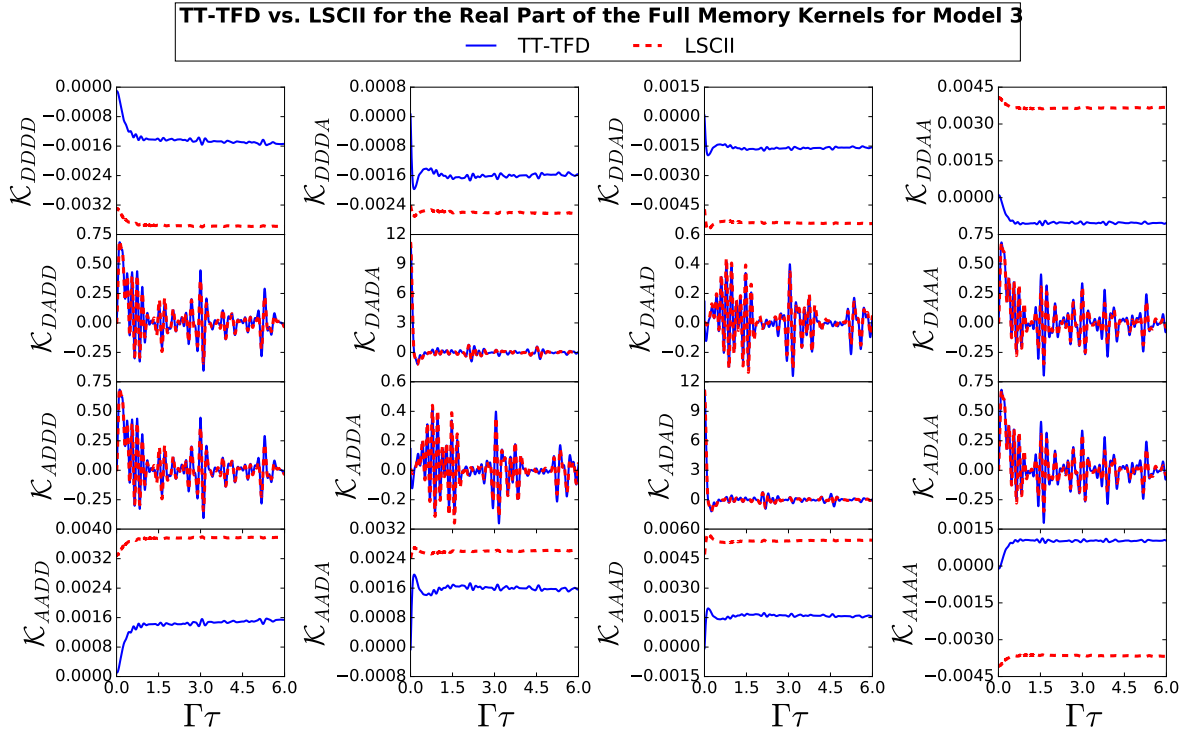

Figure S21: Real parts of the matrix elements of the memory kernel of the GQME for the full electronic density matrix  $[\mathcal{K}^{\text{full}}(\tau)]$  for model 3 as obtained from TT-TFD-based PFIs (solid blue lines) and LSCII-based PFIs (dashed red lines).

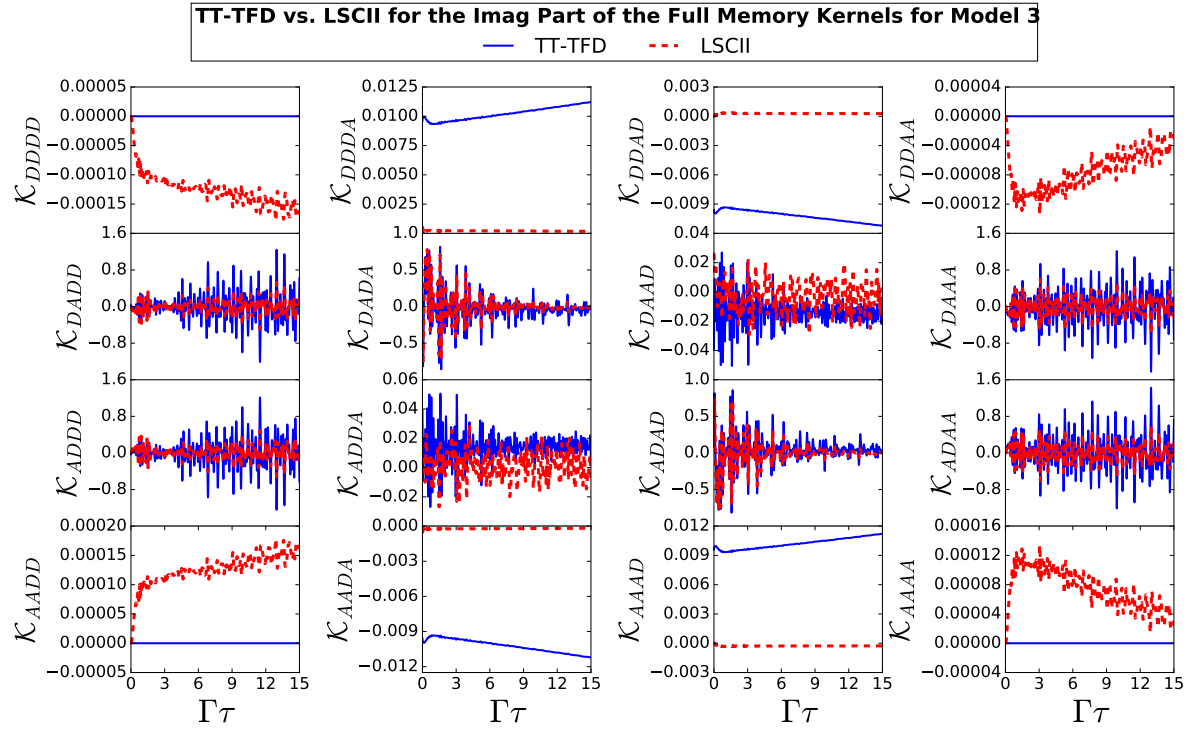

Figure S22: Imaginary parts of the matrix elements of the memory kernel of the GQME for the full electronic density matrix  $[\mathcal{K}^{\text{full}}(\tau)]$  for model 3 as obtained from TT-TFD-based PFIs (solid blue lines) and LSCII-based PFIs (dashed red lines).

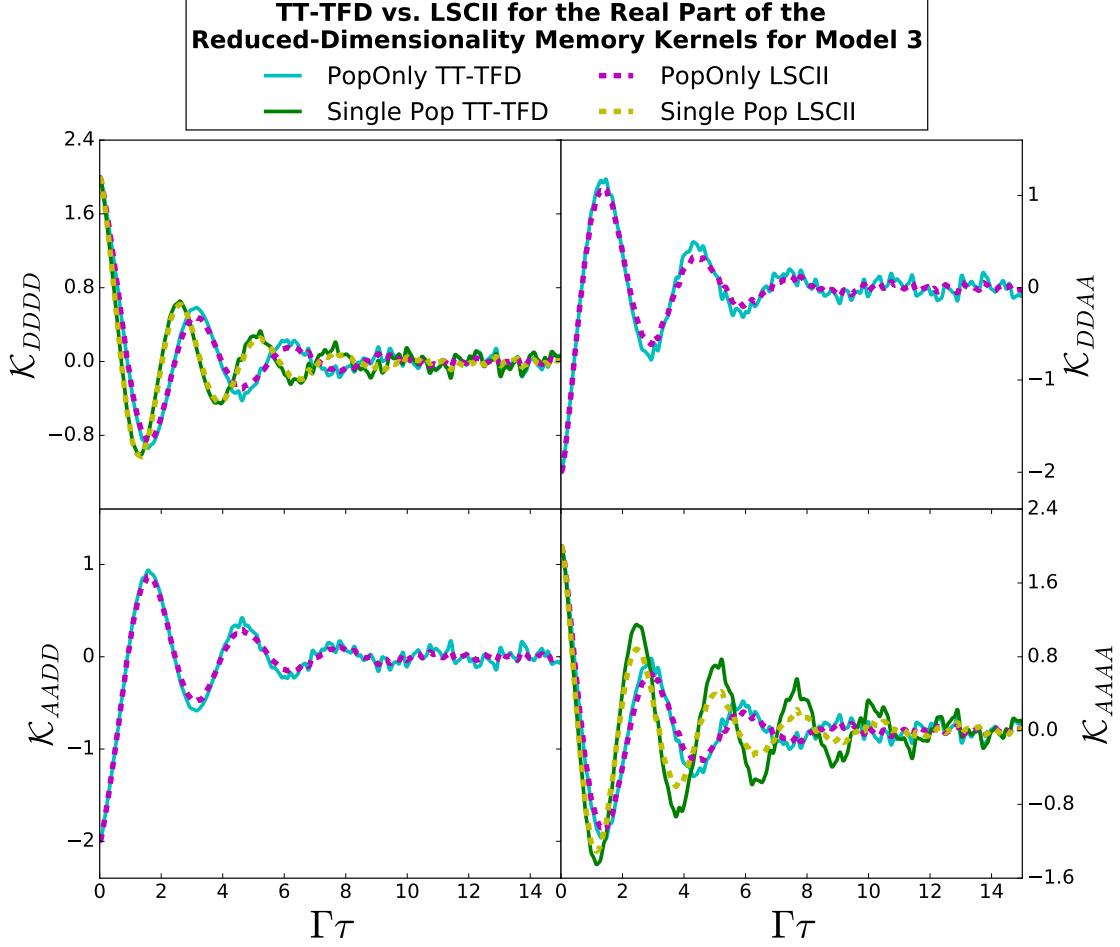

Figure S23: The real parts of the matrix elements of the memory kernels for the populations-only and single-population GQMEs for model 3 as obtained from TT-TFD-based PFIs and LSCII-based PFIs. Shown are the matrix elements of three different memory kernels: (1) The memory kernel of the populations-only GQME [ $\mathcal{K}^{\text{pop}}(\tau)$ ], which has four elements ( $DDDD, DDAA, AADD, AAAA$ ) and is depicted with solid cyan lines for the results from TT-TFD-based PFIs and dashed magenta lines for the results from LSCII-based PFIs; (2) and (3) The single-element memory kernels of the scalar single-population GQMEs [ $\mathcal{K}_{DD,DD}^{\text{donor}}(\tau)$  and  $\mathcal{K}_{AA,AA}^{\text{acceptor}}(\tau)$ ], which are depicted in the  $DDDD$  and  $AAAA$  panels, respectively, with solid green lines for the results from TT-TFD-based PFIs and dashed yellow lines for the results from LSCII-based PFIs.

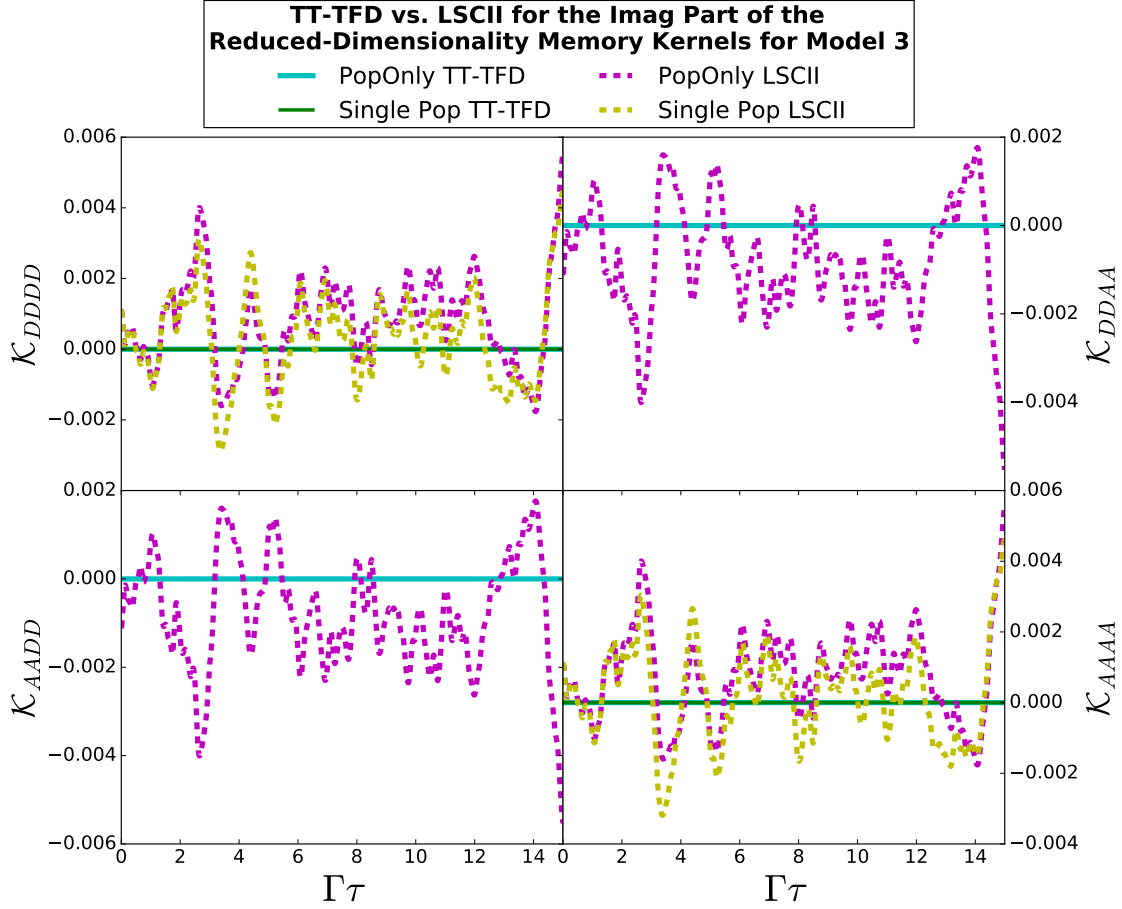

Figure S24: The imaginary parts of the matrix elements of the memory kernels for the populations-only and single-population GQMEs for model 3 as obtained from TT-TFD-based PFIs and LSCII-based PFIs. Shown are the matrix elements of three different memory kernels: (1) The memory kernel of the populations-only GQME [ $\mathcal{K}^{\text{pop}}(\tau)$ ], which has four elements ( $DDDD, DDAA, AADD, AAAA$ ) and is depicted with solid cyan lines for the results from TT-TFD-based PFIs and dashed magenta lines for the results from LSCII-based PFIs; (2) and (3) The single-element memory kernels of the scalar single-population GQMEs [ $\mathcal{K}_{DD,DD}^{\text{donor}}(\tau)$  and  $\mathcal{K}_{AA,AA}^{\text{acceptor}}(\tau)$ ], which are depicted in the  $DDDD$  and  $AAAA$  panels, respectively, with solid green lines for the results from TT-TFD-based PFIs and dashed yellow lines for the results from LSCII-based PFIs.

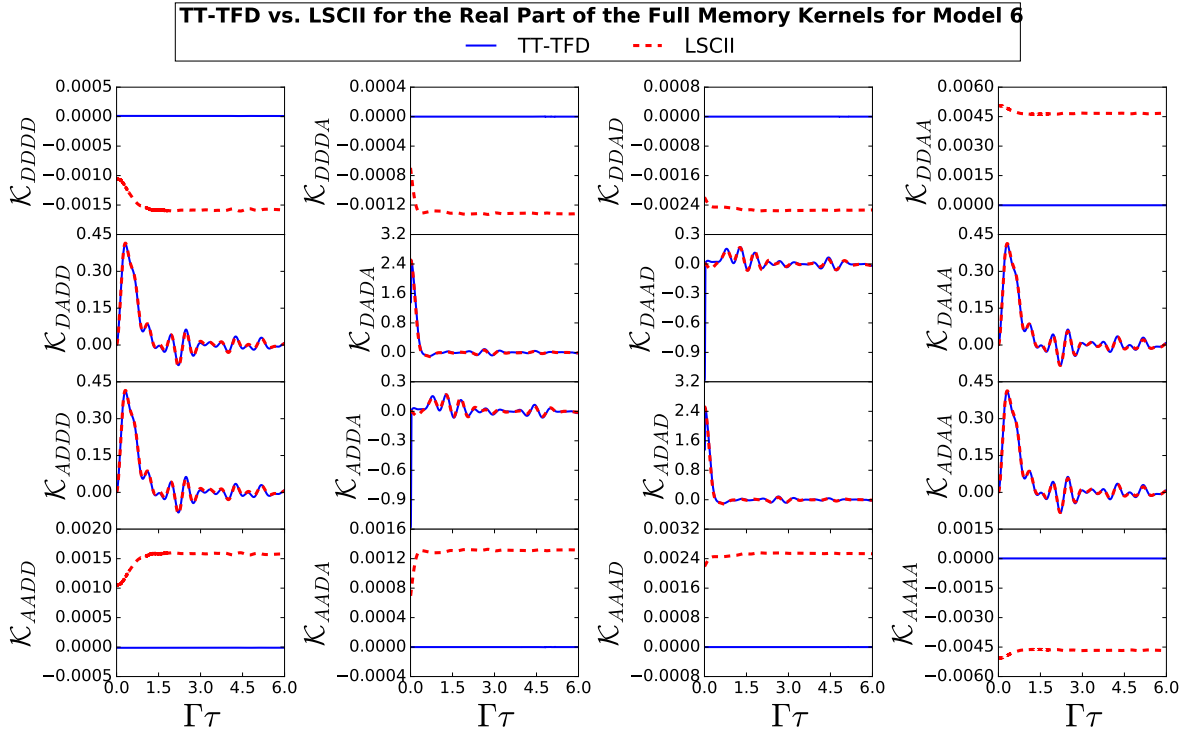

Figure S25: Real parts of the matrix elements of the memory kernel of the GQME for the full electronic density matrix  $[\mathcal{K}^{\text{full}}(\tau)]$  for model 6 as obtained from TT-TFD-based PFIs (solid blue lines) and LSCII-based PFIs (dashed red lines).

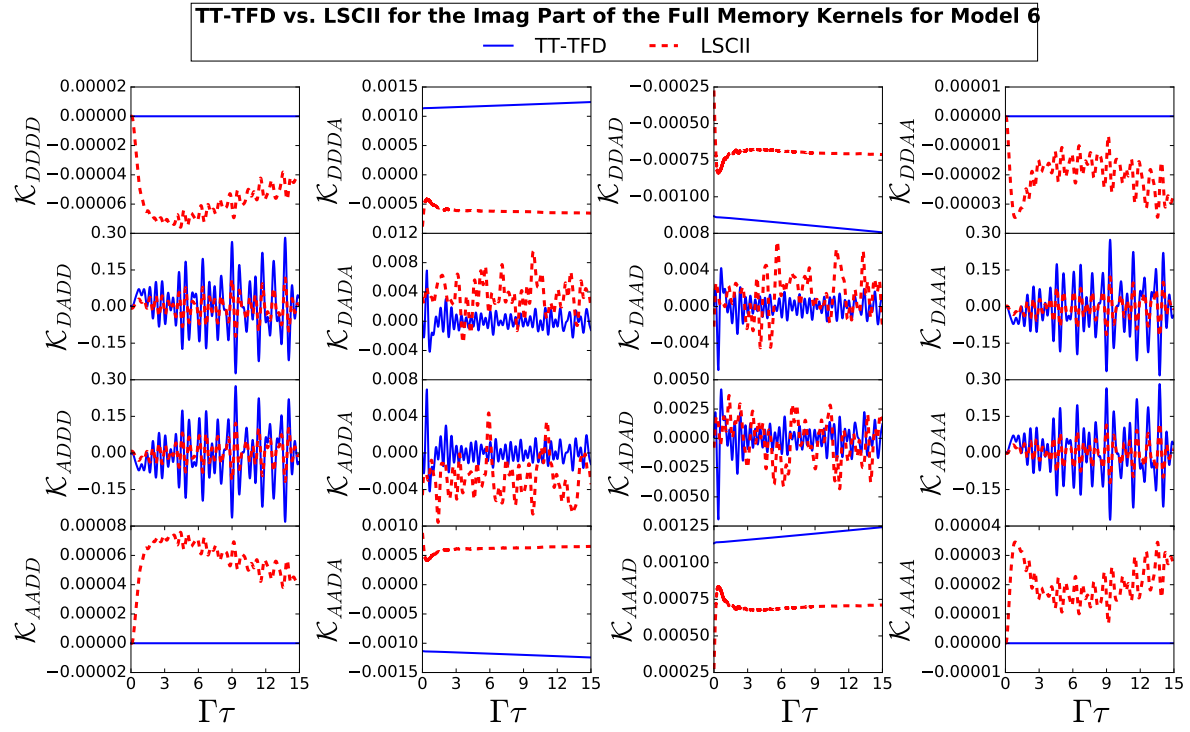

Figure S26: Imaginary parts of the matrix elements of the memory kernel of the GQME for the full electronic density matrix  $[\mathcal{K}^{\text{full}}(\tau)]$  for model 6 as obtained from TT-TFD-based PFIs (solid blue lines) and LSCII-based PFIs (dashed red lines).

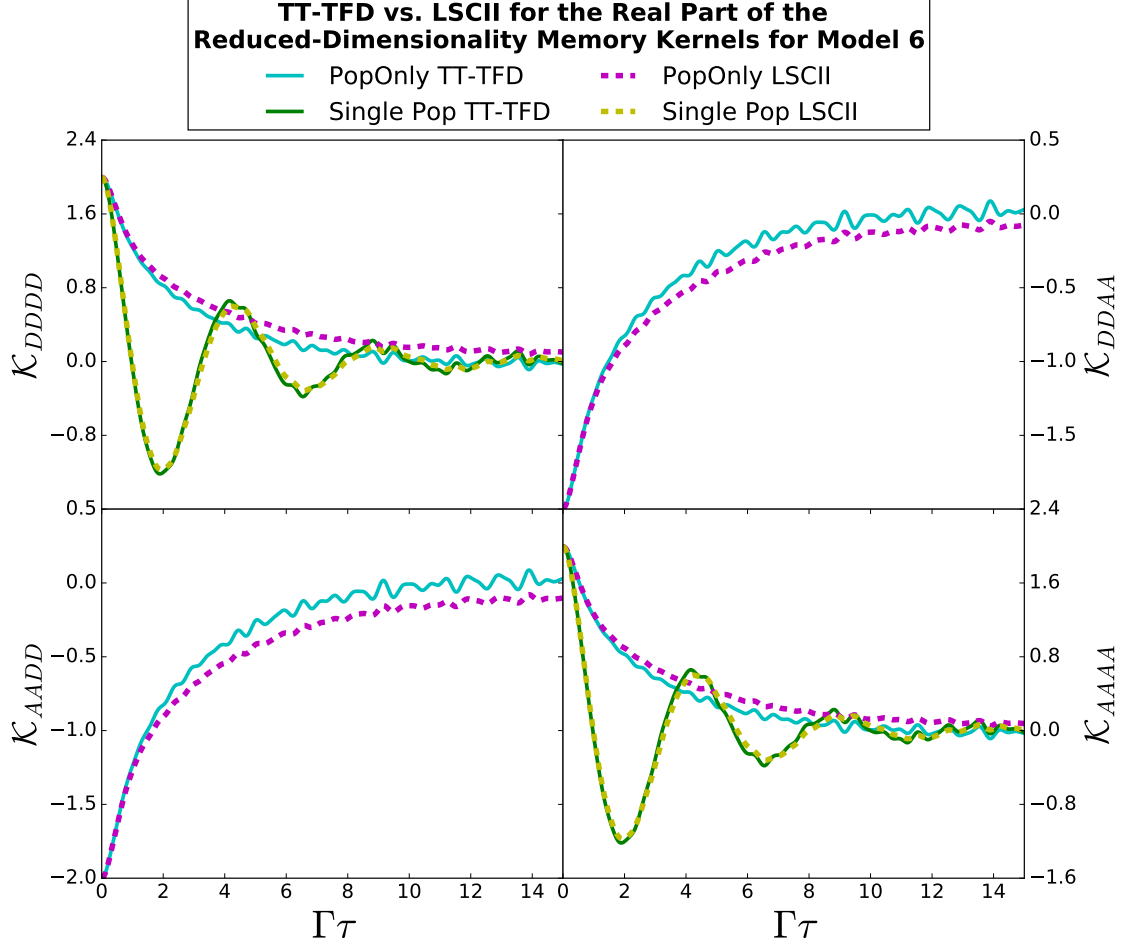

Figure S27: The real parts of the matrix elements of the memory kernels for the populations-only and single-population GQMEs for model 6 as obtained from TT-TFD-based PFIs and LSCII-based PFIs. Shown are the matrix elements of three different memory kernels: (1) The memory kernel of the populations-only GQME [ $\mathcal{K}^{\text{pop}}(\tau)$ ], which has four elements ( $DDDD, DDAA, AADD, AAAA$ ) and is depicted with solid cyan lines for the results from TT-TFD-based PFIs and dashed magenta lines for the results from LSCII-based PFIs; (2) and (3) The single-element memory kernels of the scalar single-population GQMEs [ $\mathcal{K}_{DD,DD}^{\text{donor}}(\tau)$  and  $\mathcal{K}_{AA,AA}^{\text{acceptor}}(\tau)$ ], which are depicted in the  $DDDD$  and  $AAAA$  panels, respectively, with solid green lines for the results from TT-TFD-based PFIs and dashed yellow lines for the results from LSCII-based PFIs.

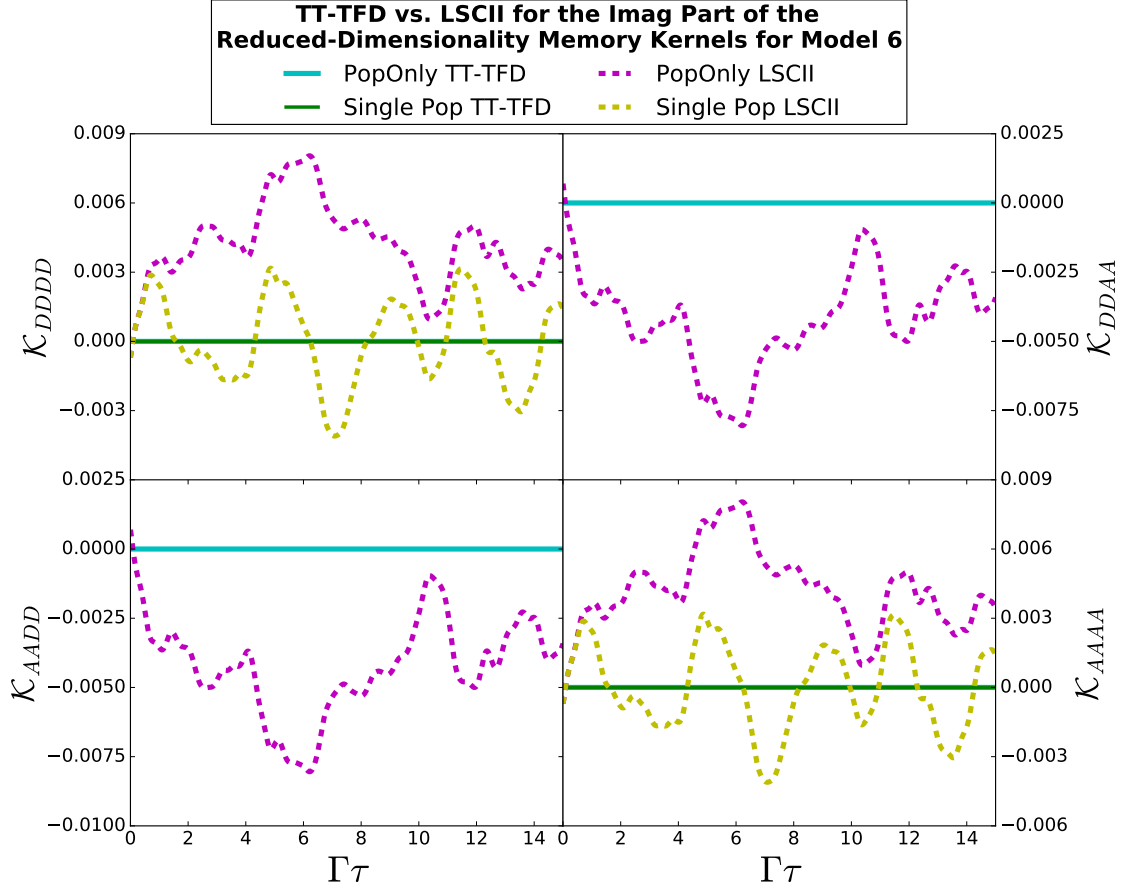

Figure S28: The imaginary parts of the matrix elements of the memory kernels for the populations-only and single-population GQMEs for model 6 as obtained from TT-TFD-based PFIs and LSCII-based PFIs. Shown are the matrix elements of three different memory kernels: (1) The memory kernel of the populations-only GQME [ $\mathcal{K}^{\text{pop}}(\tau)$ ], which has four elements ( $DDDD$ ,  $DDAA$ ,  $AADD$ ,  $AAAA$ ) and is depicted with solid cyan lines for the results from TT-TFD-based PFIs and dashed magenta lines for the results from LSCII-based PFIs; (2) and (3) The single-element memory kernels of the scalar single-population GQMEs [ $\mathcal{K}_{DD,DD}^{\text{donor}}(\tau)$  and  $\mathcal{K}_{AA,AA}^{\text{acceptor}}(\tau)$ ], which are depicted in the  $DDDD$  and  $AAAA$  panels, respectively, with solid green lines for the results from TT-TFD-based PFIs and dashed yellow lines for the results from LSCII-based PFIs.

## S.VII Graphs of the Inhomogeneous Terms of All of the Models

Given in this section are the graphs of the real part of the inhomogeneous terms for models 1, 2, 3, and 6. The imaginary part is not shown, as it is zero for all models for both inhomogeneous terms calculated via TT-TFD and LSCII.

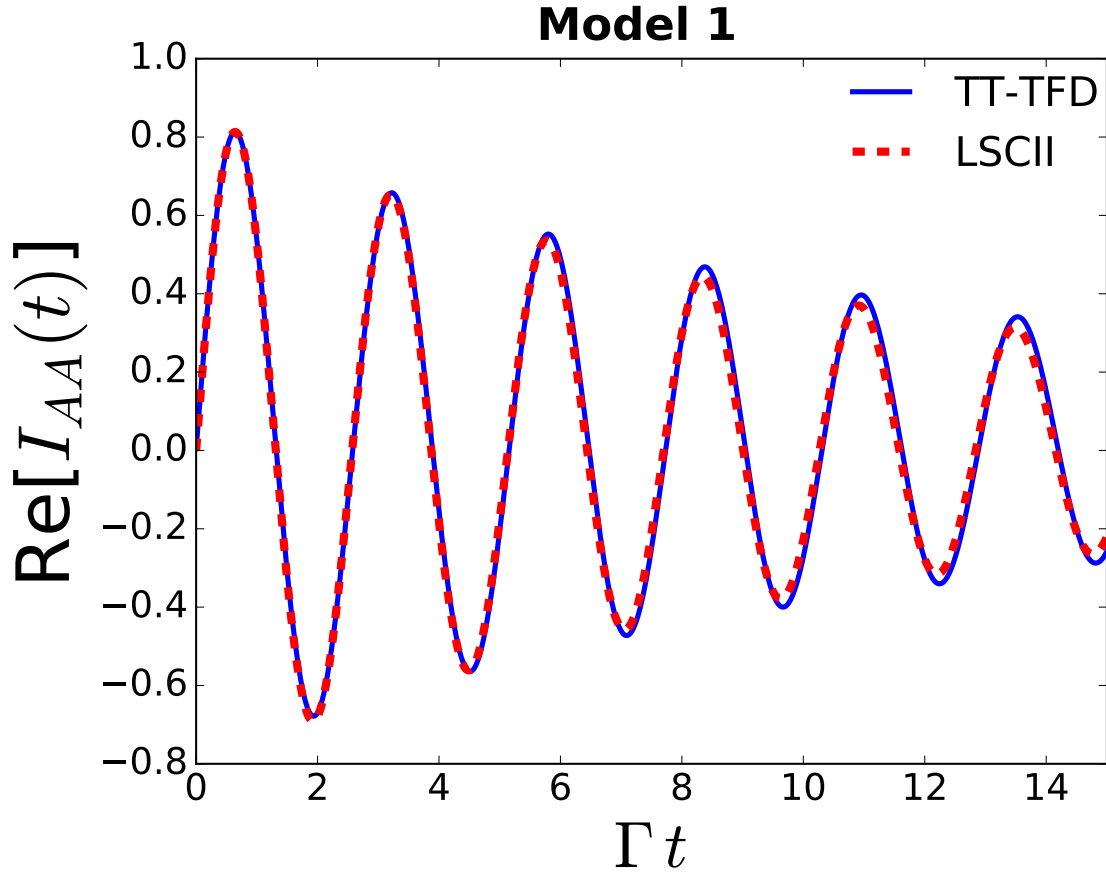

Figure S29: Real part of  $\hat{I}_{AA}(\tau)$  for model 1, as obtained from TT-TFD-based PFIs (solid blue lines) and LSCII-based PFIs (dashed red lines).

## References

- [1] R. Zwanzig, *Nonequilibrium statistical mechanics* (Oxford University Press, New York, 2001).
- [2] A. Nitzan, *Chemical Dynamics in Condensed Phases* (Oxford University Press, New York, 2006).

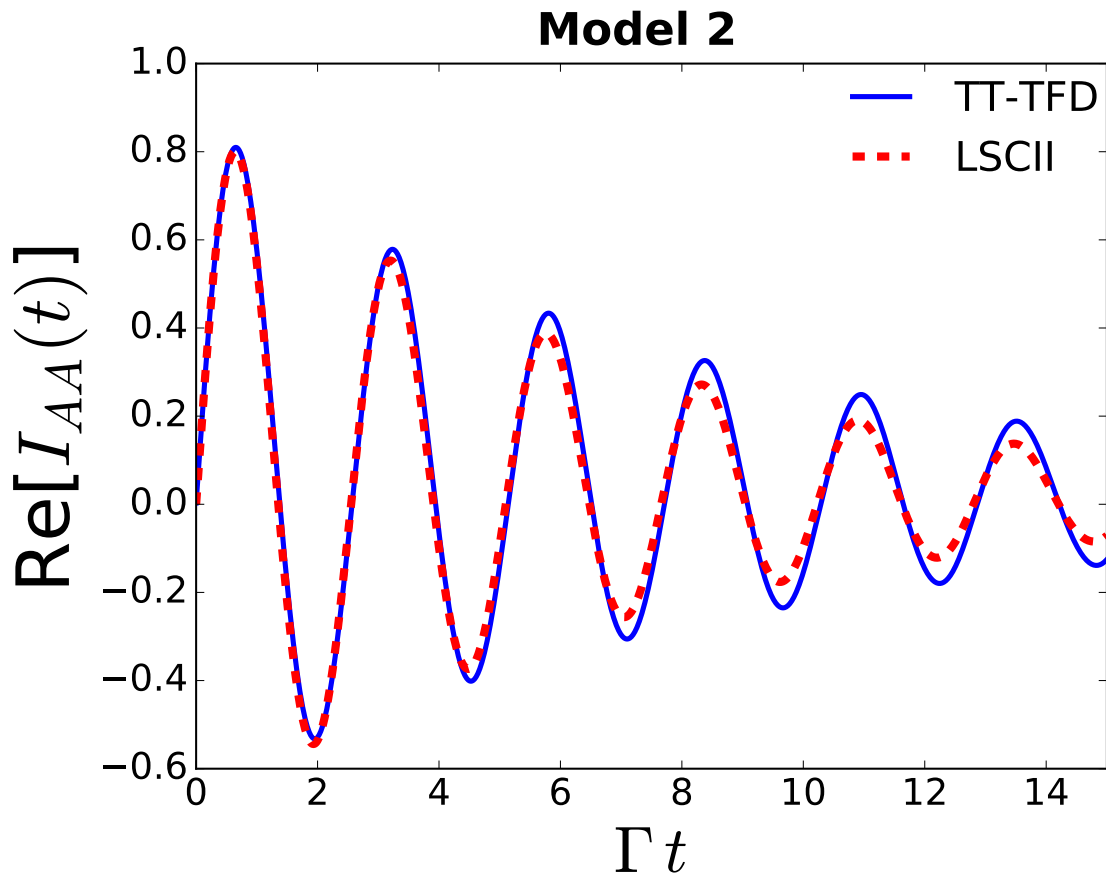

Figure S30: Real part of  $\hat{I}_{AA}(\tau)$  for model 2, as obtained from TT-TFD-based PFIs (solid blue lines) and LSCII-based PFIs (dashed red lines).

- [3] S. Mukamel, *Principles of Nonlinear Optical Spectroscopy* (Oxford, New York, 1995).
- [4] H.-P. Breuer, F. Petruccione, *The Theory of Open Quantum Systems* (Oxford Press, Oxford, 2002).
- [5] E. Mulvihill, E. Geva, *J. Phys. Chem. B* **125**, 9834 (2021).
- [6] E. Mulvihill, A. Schubert, X. Sun, B. D. Dunietz, E. Geva, *J. Chem. Phys.* **150**, 034101 (2019).
- [7] E. Mulvihill, E. Geva, *J. Chem. Phys.* **156**, 044119 (2022).
- [8] Q. Shi, E. Geva, *J. Chem. Phys.* **119**, 12063 (2003).
- [9] Q. Shi, E. Geva, *J. Chem. Phys.* **120**, 10647 (2004).
- [10] M.-L. Zhang, B. J. Ka, E. Geva, *J. Chem. Phys.* **125**, 044106 (2006).
- [11] B. J. Ka, M.-L. Zhang, E. Geva, *J. Chem. Phys.* **125**, 124509 (2006).

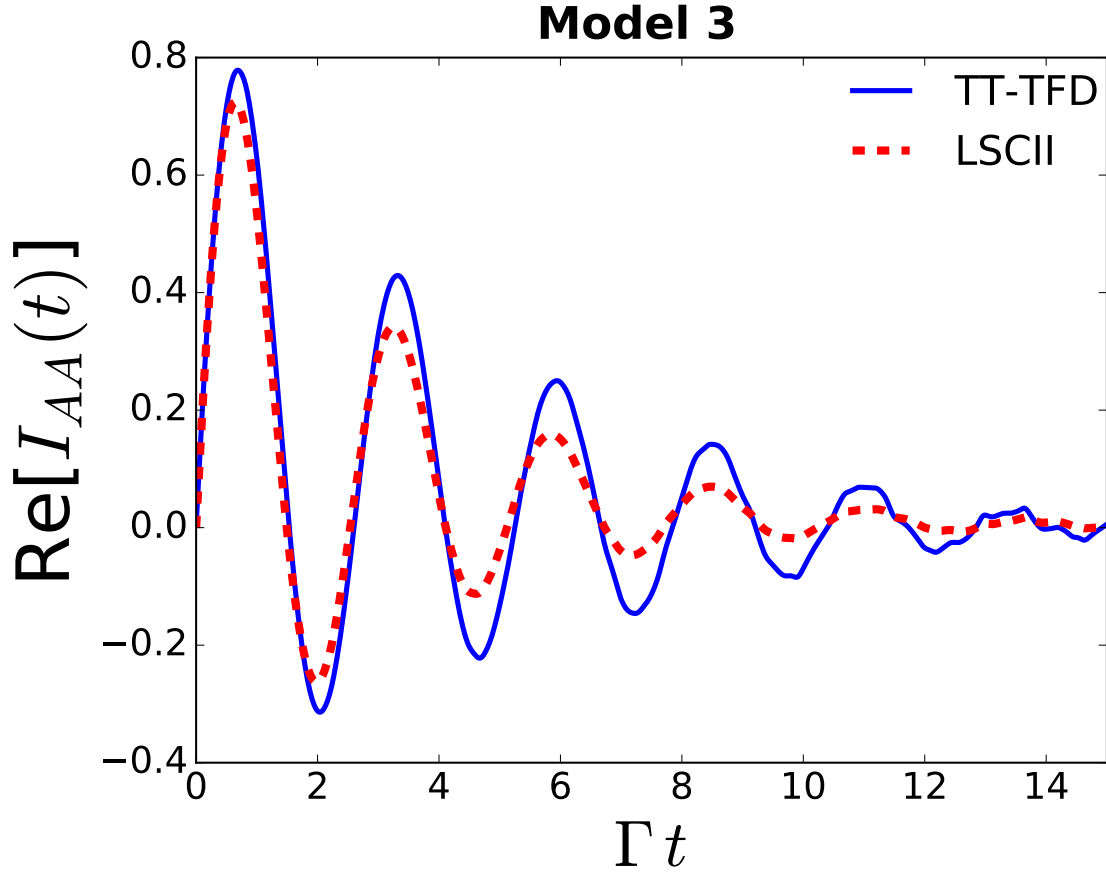

Figure S31: Real part of  $\hat{I}_{AA}(\tau)$  for model 3, as obtained from TT-TFD-based PFIs (solid blue lines) and LSCII-based PFIs (dashed red lines).

- [12] G. Cohen, E. Rabani, *Phys. Rev. B* **84**, 075150 (2011).
- [13] E. Y. Wilner, H. Wang, G. Cohen, M. Thoss, E. Rabani, *Phys. Rev. B* **88**, 045137 (2013).
- [14] G. Cohen, E. Y. Wilner, E. Rabani, *New Journal of Physics* **15**, 073018 (2013).
- [15] G. Cohen, E. Gull, D. R. Reichman, A. J. Millis, E. Rabani, *Phys. Rev. B* **87**, 195108 (2013).
- [16] A. Kelly, T. E. Markland, *J. Chem. Phys.* **139**, 014104 (2013).
- [17] L. Kidon, E. Y. Wilner, E. Rabani, *J. Chem. Phys.* **143**, 234110 (2015).
- [18] W. C. Pfalzgraff, A. Kelly, T. E. Markland, *J. Phys. Chem. Lett.* pp. 4743–4748 (2015).
- [19] A. Montoya-Castillo, D. R. Reichman, *J. Chem. Phys.* **144**, 184104 (2016).
- [20] A. Kelly, N. Brackbill, T. E. Markland, *J. Chem. Phys.* **142**, 094110 (2015).

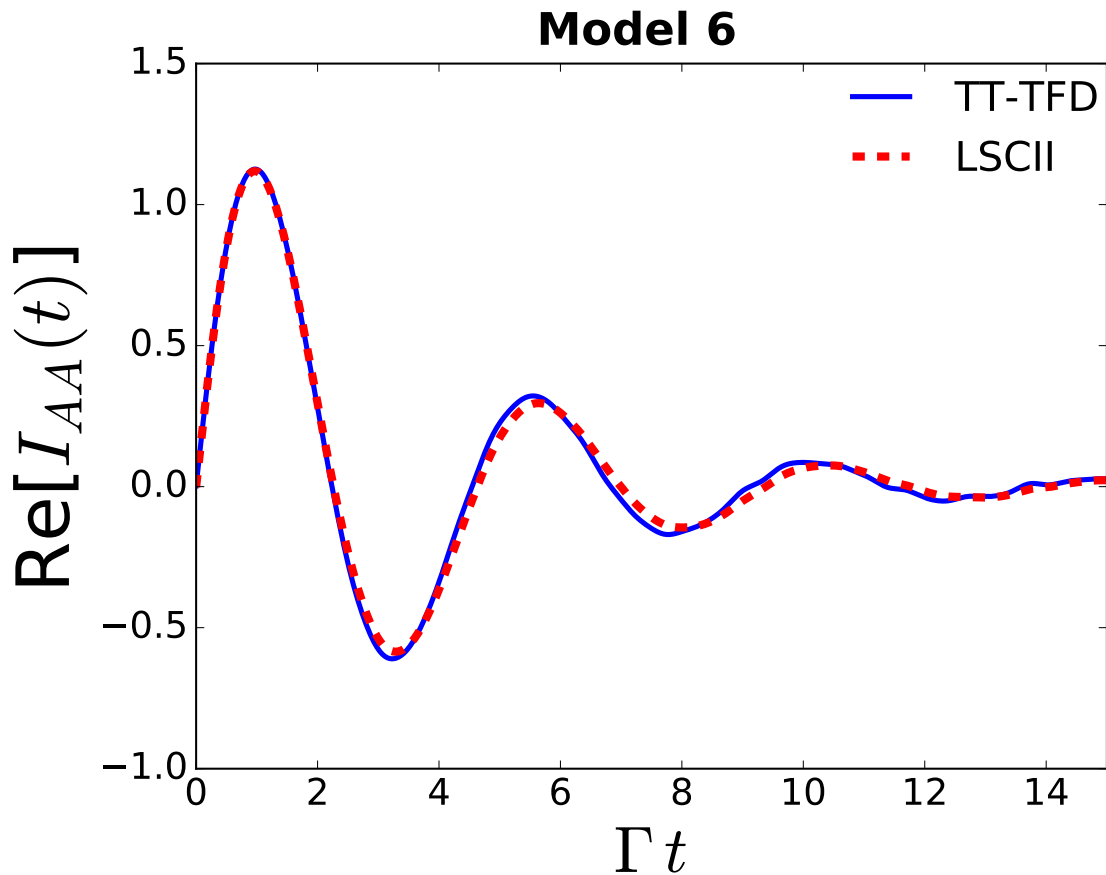

Figure S32: Real part of  $\hat{I}_{AA}(\tau)$  for model 6, as obtained from TT-TFD-based PFIs (solid blue lines) and LSCII-based PFIs (dashed red lines).

- [21] A. Kelly, A. Montoya-Castillo, L. Wang, T. E. Markland, *The Journal of Chemical Physics* **144**, 184105 (2016).
- [22] L. Kidon, H. Wang, M. Thoss, E. Rabani, *The Journal of chemical physics* **149**, 104105 (2018).
- [23] W. Pfalzgraff, A. Montoya-Castillo, A. Kelly, T. Markland, *J. Chem. Phys.* **150**, 244109 (2019).
- [24] E. Mulvihill, *et al.*, *J. Chem. Phys.* **151**, 074103 (2019).
- [25] E. Mulvihill, *et al.*, *J. Chem. Phys.* **154**, 204109 (2021).
- [26] N. Ng, D. T. Limmer, E. Rabani, *The Journal of Chemical Physics* **155**, 156101 (2021).
